# Supplementary material for: Kernel Dependence Network
Source: arXiv:2011.03320 source file (2020-11-09)
Supplement: Supplementary file 1 [file A_lemma_1.tex]

\begin{appendices}
\section{Lemma \ref{lemma:lemma1}}
\label{app:lemma_1_proof}
\subsection{Assumptions and Notations of the Proof}
Since the positive and negative properties of the $\Gamma$ matrix are used throughout several proofs in the paper, we prove its properties as a lemma here. Following the convention of the paper, we are given a dataset $X \in \mathbb{R}^{N \times d}$ of $C$ classes where $N$ denotes the number of samples and $d$ the dimensions of the data. Given $C$ classes, we let $n_c$ be the number of samples in the $c$th class. Let its classification labels use one-hot encoding and denoted as $Y \in \mathbb{R}^{N \times C}$. Also let $H$ be the centering matrix defined as $H = I - \frac{1}{N} \mathbf{1}_{N \times N}$ where $\mathbf{1}_{N \times N}  \in \mathbb{R}^{N \times N}$ represents a matrix of all 1s. Since $H$ is a centering matrix, it has the property $H = H^T$. 
Lastly, let $\Gamma \in \mathbb{R}^{N \times N}$ matrix be defined as $\Gamma = HYY^TH$.

\subsection{Lemmas of the Proof}
\begin{lemma}\label{lemma:lemma1}
If the size of any single class is less than the size of the union of any other two classes, then every ($x_i, x_j$) pair of samples of the same class has a corresponding positive $\Gamma_{i,j}$ and every ($x_i, x_j$) pair of samples of different classes has a corresponding negative $\Gamma_{i,j}$.
\end{lemma}
\begin{proof}
Given $C$ classes, the total number of samples $N$ is the summation of the number of samples, $n_c$, for each class where
    \begin{equation}
    N = \sum_{c=1} n_c.
    \end{equation}
It can be easily verified that the linear kernel matrix $K = Y Y^T$ has $(i,j)$th element as 1 and 0 if the $(x_i,x_j)$ pair belong to the same and different classes respectively. It can also be easily verified that $K=K^T$. We denote the constant $\eta$ here as 
    \begin{equation}
    \eta = \mathbf{1}_N^T K \mathbf{1}_N
    \end{equation}
where $\mathbf{1}_N$ is a vector of 1s of length $N$. In other words, $\eta$ represents the cardinality of all $(x_i,x_j)$ pairs that belong to the same classes and can also be computed as 
    \begin{equation}
    \eta = \sum_{c=1} n_c^2.
    \end{equation}
We next define the degree vector as 
    \begin{equation}
    d = [d_1, d_2, ... d_N]^T = K \mathbf{1}_N
    \end{equation}
and the stacked degree matrix $D \in \mathbb{R}^{N \times N}$ as
    \begin{equation}
    D = [d, d, ...].
    \end{equation}
To clarify, the columns of $D$ consists of repeated vectors of $d$. Given these relationship, we first apply the centering matrix to $K$ and obtain
    \begin{equation}
    HK = (I - \frac{1}{N} \mathbf{1}_{N \times N})K =
    K - \frac{1}{N} D^T.
    \end{equation}
Next, we apply the centering matrix on the right hand side and obtain  
    \begin{align*}
        \Gamma = HKH &= ((HKH)^T)^T \\
        &= (H (HK)^T)^T \\
        &= (H (K - \frac{1}{N} D^T)^T)^T \\
        &= ((I - \frac{1}{N} \mathbf{1}_{N \times N}) (K^T - \frac{1}{N} D))^T \\
        &= K - \frac{1}{N} D^T - \frac{1}{N} D + 
        \frac{\eta}{N^2} \mathbf{1}_{N \times N}.
    \end{align*}
Therefore, at each element of $\Gamma$ we get
    \begin{equation}
    \Gamma_{i,j} = K_{i,j} - \frac{1}{N}(d_i + d_j) + \frac{\eta}{N^2}.
    \end{equation}
First, we assume that the $(x_i,x_j)$ pair belong to the same class of size $n_{\kappa}$, and therefore $K_{i,j}=1$, we obtain
    \begin{align*}
    \Gamma_{i,j} &= 1 - \frac{2 n_{\kappa}}{N} + \frac{\eta}{N^2}\\
    &= \frac{N^2}{N^2} - \frac{2 n_{\kappa} N}{N^2} + \frac{\eta}{N^2}.
    \end{align*}
Since we want to show that this value is always positive, the division by $N^2$ can be ignored. Hence, we obtain
    \begin{align*}
    \frac{N^2}{N^2} - \frac{2 n_{\kappa} N}{N^2} + \frac{\eta}{N^2} &> 0 \\
    N^2 - 2 n_{\kappa} N + \eta &> 0\\
    \left[\sum_{c=1} n_c\right]\left[\sum_{c=1} n_c\right] - 2 n_{\kappa} \sum_{c=1} n_c + \sum_{c=1} n_c^2 &> 0
    \end{align*}
Since $\sum_{c=1} n_c^2$ is always positive, it is always greater than 0. For now we ignore this term and focus on proving the following inequality.
    \begin{align*}
    \left[\sum_{c=1} n_c\right]\left[\sum_{c=1} n_c\right] >& 2 n_{\kappa} \left[ \sum_{c=1} n_c \right] \\
    \left[\sum_{c=1} n_c\right] >& 2 n_{\kappa}  \\
    n_1 + n_2 + ... + n_k + ... + n_C > &2n_k\\
    n_1 + n_2 + ... + 0 + ... + n_C >& n_k
    \end{align*}
Since $n_k$ by assumption cannot be greater than the summation of any 2 classes, the above inequality is always true.

Next, we show that if $(x_i,x_j)$ are not in the same class, the $\Gamma_{i,j}$ value is always negative. In this case, $K_{i,j} = 0$ and therefore, we get
    \begin{align*}
    \Gamma_{i,j} &= 0 - \frac{1}{N}(d_i + d_j) + \frac{\eta}{N^2} \\
    &= \frac{\eta}{N^2} - \frac{N}{N^2}(d_i + d_j) .
    \end{align*}
Again, we can ignore the denominator. We let samples $x_i$ and $x_j$ come from two distinct class group of sizes $n_\alpha$ and $n_\beta$. To obtain a negative value for $\Gamma_{i,j}$ we need to satisfy the inequality 
    \begin{align*}
    \eta - N(d_i + d_j) &< 0\\
    \sum_{c=1} n_c^2 - (n_\alpha + n_\beta)(\sum_{c=1} n_c) &< 0 \\
    (n_\alpha^2 + n_\beta^2)
    - (n_\alpha^2 + n_\beta^2)
    - 2(n_\alpha n_\beta)
    - \sum_{c=1} n_c(n_c - n_\alpha - n_\beta) &< 0 \\
    - 2(n_\alpha n_\beta)
    - \sum_{c=1} n_c(n_c - n_\alpha - n_\beta) &< 0
    \end{align*}
Since $-2(n_\alpha n_\beta)$ is always negative, we can ignore this term. In fact, since $n_c$ is always positive, we can also remove it from the 2nd term and simply need to show that for all $c$
    \begin{align*}
        n_c - n_\alpha - n_\beta &< 0, \\
        n_c &< n_\alpha + n_\beta. 
    \end{align*}

Since the size of any class is always smaller than the size of the union any two classes, the inequality must be true.
Hence, its corresponding $\Gamma_{i,j}$ will also always be negative.
\end{proof}

It is important to note that our proof is simply a theoretical exercise to match the formulation with HSIC. In practice, since the labels are known, $\Gamma_{i,j}$ can always be set to 1 and -1 based on the label. This is equivalent to changing the definition of the one-hot encoded labels. Therefore, the assumption that any class cannot be larger than the combination of any other two classes can be easily circumvented if the data is highly unbalanced. In general, this proof recommends to set $\Gamma_{i,j}$ directly to positive and negative 1 instead of relying on the centering matrix.  
\end{appendices}
