# Supplementary material for: Kernel Dependence Network
Source: arXiv:2011.03320 source file (2020-11-09)
Supplement: Supplementary file 2 [file a_HSIC_objective.tex]

\begin{appendices}
\section{Proof for Theorem \ref{thm:CCN_becomes_HSIC}}
\label{app:proof_for_CCN_becomes_HSIC}

Let $R_{l-1} \in \mathbb{R}^{n \times m}$ be the input of a layer, $R_{l} \in \mathbb{R}^{n \times m}$ the output of a layer, $W_l \in \mathbb{R}^{m \times q}$ its layer weights and $\Psi$ the activation function. We also let $H$ be the centering matrix defined as $H = I - \frac{1}{n} \mathbf{1}_{n\times n}$.
A layer of MLP is equivalent to a single cyclic transition of our model starting from RKHS as showing in Fig.~\ref{fig:flow}. 
    \begin{figure}[!h]
    \centering
        \includegraphics[width=4cm,height=1.5cm]{{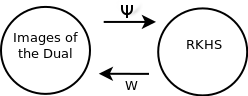}}
        \caption{Flow of information}
        \label{fig:flow}
    \end{figure}  

The dependence between $R_l = \Psi(R_{l-1} W_l)$ and its label $Y$ can be maximized by maximizing norm squared of their Cross Covariance Matrix. The Cross Covariance Matrix empirically can be computed with
    \begin{equation}
        Cov = \frac{1}{n-1}\Psi(R_{l-1}W_l)^TH H Y.
    \end{equation}
We further condense the Cross Covariance Matrix into a single value by finding its norm squared. Coincidentally, this matches the definition of HSIC in RKHS where
    \begin{equation}
        \hsic(R_{l-1}W_l) = 
        ||Cov||^2 = \frac{1}{(n-1)^2} \Tr(
        Y^T H H \Psi(R_{l-1}W_l)
        \Psi(R_{l-1}W_l)^TH H Y).
    \end{equation}
Note that since $H = HH$ and $H = H^T$, we can further condense the expression into
    \begin{equation}
        \hsic(R_{l-1}W_l) = 
        ||Cov||^2 = \frac{1}{(n-1)^2} \Tr(
        H\Psi(R_{l-1}W_l)
        \Psi(R_{l-1}W_l)^T HYY^T).
    \end{equation}
Since $YY^T$ is simply the kernel matrix for $Y$, we denote it as $K_Y$. Similarly, we also obtain the kernel matrix $K_{R_{l-1}W_l} = \Psi(R_{l-1}W_l) \Psi(R_{l-1}W_l)^T$, thereby yielding the standard HSIC objective
    \begin{equation}
        \hsic(R_{l-1}W_l) = 
        ||Cov||^2 = \frac{1}{(n-1)^2} \Tr(
        HK_{R_{l-1}W_l} H K_Y).
    \end{equation}
At this point, our goal is to discover the optimal network weight $W_l$ constrained on $W^TW=I$ at the $l$th layer that maximizes this dependency between $\Psi(R_{l-1}W_l)$ and $Y$, therefore, we arrive to our objective Eq.~(\ref{eq:hsic_obj_pure}) where
    \begin{equation}
        \underset{W_l}{\max} \quad \Tr( HK_Y H K_{R_{l-1} W_l} )
        \hspace{0.3cm} \text{s.t} \hspace{0.3cm} W_l^TW_l = I.
    \end{equation}
\end{appendices}
