# Supplementary material for: Kernel Dependence Network
Source: arXiv:2011.03320 source file (2020-11-09)
Supplement: Supplementary file 3 [file a_thm_1_2.tex]

\begin{appendices}
\section{Proof for Proposition \ref{thm:central_theorem}}
\label{app:central_theorem}
\textbf{Theorem} \ref{thm:central_theorem} :
\textit{ If each cyclic transition is greedily optimized to generate a monotonic sequence in a bounded space, then Properties~\ref{prop:convergent_property} and \ref{prop:convergent_limit_property} are satisfied.}

\begin{proof}
To begin our proof, we first evoke the Monotone Convergence Theorem \cite{bibby1974axiomatisations} which states that a monotone sequence is guaranteed to have a limit if and only if the sequence is bounded. 
Since this condition is assumed to be true in Theorem \ref{thm:central_theorem}, then it follows that the sequence generated by the cyclic transitions must also converge to a limit. Hence, Property~\ref{prop:convergent_property} is satisfied.

As for Property 2, the limit of the sequence must satisfy the 2nd order condition. By assuming that the MLP is solved greedily, this implies that the output of the previous layer is used as input for the next layer. Therefore, each cycle is its own optimization problem. Assuming that each cyclic transition is solved to satisfy the 2nd order condition, then every element of the \textit{risk sequence} must also satisfy the 2nd order condition. Therefore guaranteeing the limit of the sequence to satisfy the 2nd order condition and Property 2.
\end{proof}
\end{appendices}
