# Supplementary material for: Kernel Dependence Network
Source: arXiv:2011.03320 source file (2020-11-09)
Supplement: Supplementary file 4 [file b_hsic_is_affinity.tex]

\begin{appendices}
\section{Proof for Theorem \ref{thm:ccn_satisfies_dependence_property}}
\label{app:ccn_satisfies_dependence_property}
\textbf{Theorem} \ref{thm:ccn_satisfies_dependence_property}:  
\textit{HSIC is an affinity objective}.  

\begin{proof}
Given $\mathcal{S}$ and $\mathcal{S}^c$ as sets of all pairs of samples of $(x_i,x_j)$ from a dataset $X$ with labels $Y$ that belongs to the same and different classes respectively, let $\Gamma_{i,j}$ be a set of scalar values, and let $\kappa$ be a similarity measure between any pairs of $(x_i, x_j)$. 

To prove Theorem~\ref{thm:ccn_satisfies_dependence_property}, we first leverage the result from \citet{gretton2005measuring} and rewrite the CCN objective as  
\begin{equation}
    \underset{W}{\max} \quad \Tr( K_{XW} H K_Y H)
    \hspace{1cm} \text{s.t} \hspace{1cm} W^TW = I.
     \label{eq:in_appendix_hsic_trace_obj}
\end{equation}
    If we let $\Gamma = HK_YH$ and convert the trace into a sum, then Eq.~(\ref{eq:in_appendix_hsic_trace_obj}) becomes
    \begin{equation}
        \underset{W}{\max} \quad \sum_{i,j} \Gamma_{i,j} K_{(XW)_{i,j}}
        \hspace{1cm} \text{s.t} \hspace{1cm} W^TW = I.
         \label{eq:in_appendix_hsic_sum}
    \end{equation}
    By the definition of kernel matrices, $K_{(XW)_{i,j}}$ is the inner product of $\Psi(W^Tx_i)$ and $\Psi(W^Tx_j)$, or $\langle \Psi(W^Tx_i), \Psi(W^Tx_j) \rangle$. By applying Lemma~\ref{lemma:lemma1} in Appendix~\ref{app:lemma_1_proof}, 
    Eq.~(\ref{eq:in_appendix_hsic_sum}) can be split into positive and negative $\Gamma_{i,j}$s where 
     \begin{equation}
        \underset{W}{\max} \quad \sum_{i,j \in \mathcal{S}} \Gamma_{i,j} 
        \langle \Psi(W^Tx_i), \Psi(W^Tx_j) \rangle - 
        \sum_{i,j \in \mathcal{S}^c}
        \Gamma_{i,j} 
        \langle \Psi(W^Tx_i), \Psi(W^Tx_j) \rangle
        \hspace{0.2cm} \text{s.t} \hspace{0.2cm} W^TW = I.
    \end{equation}   
    Since the inner product between unit vectors is a similarity measure of the angular distance, by setting $\kappa(. , .)$ as the inner product and letting $f = \Psi \circ W$ the theorem is proven.
\end{proof}
\end{appendices}
