# Supplementary material for: Kernel Dependence Network
Source: arXiv:2011.03320 source file (2020-11-09)
Supplement: Supplementary file 5 [file b_thm2_redo.tex]

\begin{appendices}
\section{Proof for Theorem \ref{thm:the_right_activation_function}}
\label{app:the_right_activation_function}
Given:
    \begin{equation}
        \min_{W_l} \quad -\hsic(R_{l-1}W_l, Y) \quad
        \st W_l^TW_l = I.
        \label{eq:app:hsic}
    \end{equation}
    
\textbf{Theorem \ref{thm:the_right_activation_function}: }
    \textit{Given a \textbf{risk sequence} of globally optimized empirical risks $(\mathcal{E}_1^*, ..., \mathcal{E}_L^*)$ that is individually generated via the Greedy method with Eq.~(\ref{eq:app:hsic}) as proposed by Algorithm 1. If a RBF kernel is used, the \textbf{risk sequence} monotonically decreases and converges.}

\subsection{Assumptions and Notations of the Proof}

\begin{addmargin}[1em]{2em}% 1em left, 2em right
    Here, we let $R_{l-1}$ be the input to the $l$th layer where $r_i$ represents the $i$th sample of $R_{l-1}$.
    Given $W_l$ as the weight of the $l$th layer and let the non-linear activation function at the $l$th layer is denoted as $\phi_l$. Given $\mathcal{S}$ and $\mathcal{S}^c$ as sets of all pairs of samples of $(r_i,r_j)$ from a dataset $R_{l-1}$ that belongs to the same and different classes respectively. Corresponding to the data matrix $R_{l-1}$ is the label matrix $Y \in \mathbb{R}^{n \times c}$ where $c$ denotes the number of classes. Each label $y_i \in \mathbb{R}^c$ is in the one-hot encoding format. 
    
    We also here note the definition of an injective mapping, i.e., $\phi$ is injective if
    \begin{equation}
        x_{i} \neq x_{j} \rightarrow \phi(x_{i}) \neq \phi(x_{j}).
    \end{equation} 
    
 Although there are many ways to generate converging sequences, here, we leverage the 
Monotone Convergence Theorem \cite{bibby1974axiomatisations} where a monotone sequence is guaranteed to have a limit if and only if the sequence is bounded. Therefore, if each transition generates an $\mathcal{E}_l$ lower than $\mathcal{E}_{l-1}$ in a bounded space, the \textit{risk sequence} is guaranteed to converge, i.e., the monotonic decrease of the \textit{risk sequence} directly implies a convergence.

If we let $\Gamma = HK_YH$, then Eq.~(\ref{eq:app:hsic}) can be reformulated into
\begin{equation}
    \max_{W_l} \sum_{i,j} \Gamma_{i,j} K_{R_{l-1}W_{l_{i,j}}} \quad
    \st W_l^TW_l = I.
    \label{eq:app:hsic_sum}
\end{equation}
Since $\Gamma_{i,j}$ came directly from the label, it is a bounded value, i.e, the elements of th $\Gamma$ matrix is bounded. In addition, since the kernel matrix is the inner product of the elements in RKHS, and each function is bounded in $L_2$, the kernel matrix itself is also bounded. Together, the empirical risk $\mathcal{E} = \sum_{i,j} \Gamma_{i,j} K_{R_{l-1}W_{l_{i,j}}}$ must also exist in a bounded space. Since the space for $\mathcal{E}$ is bounded, the key to prove Thm.~\ref{thm:the_right_activation_function} is to demonstrate the monotonicity of \textit{risk sequence} by confirming the inequality 
\begin{equation}
    \mathcal{E}^*_l \ge \mathcal{E}^*_{l+1}.
    \label{eq:app:inequal}
\end{equation}
Since the empirical risks at local minimums can vary wildly, for theoretical analysis purpose, we assume that the sequence is generated only at the global minimum at each stage. In addition, we assume that an algorithm capable of obtaining the global is given. Specifically, we assume to be given an algorithm capable of solving Eq.~(\ref{eq:app:hsic}) while satisfying the First and Second Order Necessary Conditions as defined by \citet{bertsekas1997nonlinear}. Given these assumption, the contribution of the prove is to show that in an ideal case, applying the feature map of RBF kernels as the non-linearity of a network layer leads to a sequence that satisfies Inequality~(\ref{eq:app:inequal}).
\end{addmargin}

\begin{proof}
We first note that $f_{l^\circ} = f_l \circ f_{l-1} \circ ... \circ f_1$, therefore the globally optimal argument of Eq.~(\ref{eq:app:hsic_sum}) can be rewritten and solved as
\begin{equation}
    W_l^* = \argmax_{W_l} \quad
    \sum_{i,j} \Gamma_{i,j} 
    \langle
        f_{l^\circ}(x_i), f_{l^\circ}(x_j)
    \rangle
    \quad
    \st W_l^TW_l = I.
    \label{eq:app:hsic_sum}
\end{equation}
If we let the set $\mathcal{Q}_{l}$ be the space of potential $W$ matrices for Eq.~(\ref{eq:app:hsic_sum}), then $W^*_l$ is the optimal $W$ at layer $l$ within the set $\mathcal{Q}_l$. Next, if we let $\mathcal{Q}_{l+1}$ be the space of potential $W$ matrices at the $l+1$ layer. If we can show that $W^*_l$ is also inside the set of $\mathcal{Q}_{l+1}$, then the best $W$ matrix in $\mathcal{Q}_{l+1}$ must be at least as good as $W^*_l$, and therefore, $\mathcal{E}^*_l \ge \mathcal{E}^*_{l+1}$ is also true.

We next note that Eq.~(\ref{eq:app:hsic_sum}) using a RBF kernel can also be written as
\begin{equation}
    W_l^* = \argmax_{W_l} \quad
    \sum_{i,j} \Gamma_{i,j} 
    e^{-\frac{(r_i-r_j)^TW_l W_l^T(r_i-r_j)}{2\sigma^2}}
    \quad
    \st W_l^TW_l = I.
    \label{eq:app:hsic_rbf_sum}
\end{equation}
Since $\Gamma_{i,j}$ is positive for all $(r_i,r_j) \in \mathcal{S}$ and negative for $(r_i,r_j) \in \mathcal{S}^c$, Eq.~(\ref{eq:app:hsic_rbf_sum}) can be further broken into 
\begin{equation}
    W_l^* = \argmax_{W_l} \quad
    \underbrace{ 
    \sum_{i,j \in \mathcal{S}} \Gamma_{i,j} 
    e^{-\frac{(r_i-r_j)^TW_l W_l^T(r_i-r_j)}{2\sigma^2}}
    }_\text{1st term}
    -
    \underbrace{
    \sum_{i,j \in \mathcal{S}^c} \Gamma_{i,j} 
    e^{-\frac{(r_i-r_j)^TW_l W_l^T(r_i-r_j)}{2\sigma^2}} 
    }_\text{2nd term}
    \quad
    \st W_l^TW_l = I.
    \label{eq:app:hsic_rbf_sum_split}
\end{equation}
Since the $\Gamma_{i,j}$ of Eq.~(\ref{eq:app:hsic_rbf_sum_split}) are all positive for the 1st term and negative for the 2nd term. It immediately tells us what the global optimal solution should be. Namely, we wish for the first exponential terms to all be 1s, and the 2nd expoential term to all be 0s. This solution is possible if there exists a $W_l^*$ such that 
\begin{equation}
    \underbrace{
    W_l^T(r_i-r_j) = 0}_{\text{Condition 1}} 
    \quad 
    \forall \quad (r_i,r_j) \in \mathcal{S}
\end{equation}
and
\begin{equation}
    \underbrace{
    W_l^T(r_i-r_j) > 0}_{\text{Condition 2}} 
    \quad 
    \forall \quad (r_i,r_j) \in \mathcal{S}^c
\end{equation}
    We emphasize that $W_l^T(r_i - r_j) > 0$ is a sufficient condition because $\sigma > 0$ can be set arbitrarily small for the 2nd exponential term to approach 0. Specifically, we note that if $W^*_l$ exists, then when $\sigma$ is set arbitrarily small the 1st term becomes
\begin{equation}
    \underbrace{ 
    \lim_{\sigma \to 0} 
    e^{-\frac{(r_i-r_j)^TW_l W_l^T(r_i-r_j)}{2\sigma^2}}
    }_\text{1st term} = 1 \quad
    \forall i,j \in \mathcal{S},
\end{equation}
and the 2nd term becomes
\begin{equation}
    \underbrace{ 
    \lim_{\sigma \to 0} 
    e^{-\frac{(r_i-r_j)^TW_l W_l^T(r_i-r_j)}{2\sigma^2}}
    }_\text{1st term} = 0 \quad
    \forall i,j \in \mathcal{S}^c.
\end{equation}
Therefore, as $\sigma \to 0$, $W_l^T(r_i - r_j) > 0$ and $W_l^T(r_i - r_j) >> 0$ for all $(r_i,r_j) \in \mathcal{S}^c$ produces the same empirical risk $\mathcal{E}_l$. Our theorem focuses on the usage of the RBF kernels because as $\sigma \to 0$, it simplifies each element of our \textit{risk sequence} into two possibilities when a layered is optimized: 
\begin{enumerate}
  \item Condition 1 and 2 are satisfied (global optimal solution).
  \item Condition 1 failed and condition 2 is satisfied (not global optimal solution). 
\end{enumerate}
We claim that if the $(l-1)$th layer is in the first possible situation, it will always stay in the 1st situation given the next additional layer. However if the $(l-1)$th layer is in the 2nd situation, 

having a tuning $\sigma$

allows us

is an injective mapping \cite{sriperumbudur2008injective}.

possible for $f_{l+1}$ to be an identity map, i.e., 
\begin{equation}
    f_{l+1} \circ f_l(x) = f_l(x).
    \label{eq:app:identity_map}
\end{equation}
This possibility implies that the option of not changing Eq.~(\ref{eq:app:hsic_sum}) is a potential solution when $f_{l+1}$ is added. And if not changing the equation is a option, $W^*_l$ must be within the set of $\mathcal{Q}_{l+1}$. To finalize the prove, we provide the mapping where a RBF kernel with an $W_{l+1}$ can induce a $f_{l+1}$ that is an identity map.

, i.e., if we let the feature map of a characteristic kernel be $\phi$, then there exists a $\phi^{-1}$ such that $\phi^{-1} [ \phi(R_{l-1}) ] = R_{l-1}$. Additionally, we know that $W \in \mathbb{R}^{d \times q}$ where $d$ is the dimension of its input and $q$ can range from 1 to $\infty$, $W^{-1}$ also exists in the potential solution space. Since the composition of an injective $W$ and $\phi$ forms $f_{l+1}$, an injective $f_{l+1}$ exists within the set of potential solutions. Therefore, at the $l+1$th layer, it can 
\end{proof}
\end{appendices}
