# Supplementary material for: Kernel Dependence Network
Source: arXiv:2011.03320 source file (2020-11-09)
Supplement: Supplementary file 6 [file b_thm_3.tex]

\begin{appendices}
\section{Proof for Theorem \ref{thm:the_right_activation_function}}
\label{app:the_right_activation_function}

\textbf{Theorem \ref{thm:the_right_activation_function}: }
    For Gaussian kernels,  there exist a set of weights ${W_1, ..., W_L}$ such that the CCN objective generates a uniformly converging \textit{risk sequence}

\subsection{Assumptions and Notations of the Proof}
\begin{addmargin}[1em]{2em}% 1em left, 2em right
    Given $\mathcal{S}$ and $\mathcal{S}^c$ as sets of all pairs of samples of $(x_i,x_j)$ from a dataset $X \in \mathbb{R}^{n \times d}$ that belongs to the same and different classes respectively. Corresponding to the data matrix $X$ is the label matrix $Y \in \mathbb{R}^{n \times c}$ where $c$ denotes the number of classes. Each label $y_i \in \mathbb{R}^c$ is in the one-hot encoding format. Let $\Gamma_{i,j}$ be a set of scalars, and let $\kappa$ be a similarity measure between any pairs of $(x_i, x_j)$. 
    
    By leveraging the Monotone Convergence Theorem, we know that a monotonic sequence in a bounded space converges to a fixed point. Since the solution space is bounded via the constraint of $W^TW=I$, the objective is to prove the monotonic improvements. This can be accomplished by proving the existence of a solution $W_l$ for the following inequality 
    \begin{equation}
        \underset{f_l}{\max} \quad ||\text{Cov}(f_{l^\circ}(X), Y)||_F \geq
        ||\text{Cov}(f^*_{(l-1)^\circ}(X), Y)||_F.
        \label{eq:key_inequality}
    \end{equation}
    Here, we denote $f^*_{(l-1)^\circ}$ as the optimal mapping discovered from the previous layer. The goal of the proof is to show the existence of $f_l$ such that $f_{l^\circ}$ will produce an equal or higher dependence at the current layer.
    
    Note that by using the Gaussian feature map as the activation function, the theoretical dimension of the mapping output is infinity with a norm of 1. Given an input sample $x_i$, we define $r_i$ such that $r_i = f^*_{(l-1)^\circ}(x_i)$. Following this notation, we let $R_{l-1} = [r_1, r_2, ..., r_n]^T$, therefore, $R_{l-1} = f^*_{(l-1)^\circ}(X)$ where $||r_i|| = 1$ for all $i$. In addition, by using a Gaussian kernel, the inner product between any two samples is bounded between 0 and 1 where $0 \le r_i^Tr_j \le 1$. We also leverage Dini's Theorem \cite{bartle1992introduction} in our proof, which states:
    
    \textbf{Dini's Theorem. }
    If a monotone sequence of continuous functions converges pointwise on a compact space and if the limit function is also continuous, then the convergence is uniform.

    The proof for Theorem \ref{thm:the_right_activation_function} is divided into 2 Lemmas, i.e., lemmas \ref{lemma:gaussian_equal_} and 
    \ref{lemma:exist_weights}. In the next subsection, we provide a brief summary of how each lemma combine to prove the theorem.
\end{addmargin}

\subsection{Summary of the Proof}

\begin{addmargin}[1em]{2em}% 1em left, 2em right
\textbf{In Lemma~\ref{lemma:gaussian_equal_},} we demonstrate that when a Gaussian kernel is used with HSIC, the argmax of the HSIC objective is equivalent to the argmax of an \textit{affinity objective} using a negative Euclidean distance as a similarity measure. We refer to this objective as the \textit{Euclidean Affinity} defined as
\begin{equation}
        \underset{W}{\argmax} \quad   
        \Tr(W^TA_=W)
         - 
        \Tr(W^T A_{\ne}W) 
        \hspace{0.2cm} \text{s.t} \hspace{0.2cm} W^TW = I.
       \label{eq:euclid_object} 
\end{equation}
$A_=$ is defined as 
\begin{equation}
    A_= = \frac{1}{\sigma^2} \sum_{i,j \in \mathcal{S}} (r_i - r_j)(r_i - r_j)^T,
\end{equation}
and $A_{\ne}$ is defined as 
\begin{equation}
    A_{\ne} = \frac{1}{\sigma^2}\sum_{i,j \in \mathcal{\tilde{S}}} (r_i - r_j)(r_i - r_j)^T.
\end{equation}

Therefore, instead of solving the HSIC objective directly, we can optimize the \textit{Euclidean Affinity} as a surrogate objective since the argmax for both objectives are equivalent.

\textbf{In Lemma~\ref{lemma:exist_weights},} we first define $V$ as the set of eigenvectors of $A_{\ne}$ that have positive eigenvalues. Given $V$, we show that if the null space of $A_=$ is sufficiently large to intersect with the span of $V$, then a globally optimal solution $W^*$ exists. Since the null space of $A_=$ for a Gaussian kernel is infinitely large, unless the span of $A_=$ completely overlaps the span of $V$ (not possible), an intersection always exists, i.e., a global optimal $W^*$ exists. Given the existence of $W^*$, there must also exist a set of $W$s, $\{W_1, ..., W^*\}$, sampled from interpolation points between a point within the neighborhood of $W^*$ and $W^*$ that monotonically improves the objective. Lastly, since the Gaussian kernel is a Universal kernel, all of its functions in RKHS are continuous, therefore, the monotonic convergence is also uniform.
\end{addmargin}

\subsection{Lemmas of the Proof}

\begin{lemma}\label{lemma:gaussian_equal_}
Assuming that the feature map of a Gaussian kernel is used as the activation function, then the LHS of the Inequality~(\ref{eq:key_inequality}) we denote here as 
\begin{equation}
    \underset{W}{\argmax} \quad ||\text{Cov}(\Psi(R_{l-1}W), Y)||_F 
    \quad \text{s.t : } \quad W^TW = I
    \label{eq:cov_objective2}
\end{equation}
is equivalent to Eq.~(\ref{eq:euclid_object}).
\end{lemma}

\begin{proof}
Following the proof by \citet{gretton2005measuring}, the norm of the cross-covariance can be reformulated into the empirical HSIC objective where the inequality becomes
\begin{equation}
    ||\text{Cov}(\Psi(R_{l-1}W), Y)||_F
    =
    HSIC(R_{l-1} W, Y).
\end{equation}
Therefore, optimizing the CCN objective is equivalent to solving
\begin{equation}
    \underset{W}{\argmax} \quad 
    \Tr(K_{R_l W} H K_Y H) 
    \quad \textit{s.t : } \quad W^TW = I.
\end{equation}
If we let $\Gamma_{i,j}$ be the $(i,j)th$ element of the matrix $\Gamma = HK_YH$ and write out the Gaussian kernel, the objective becomes

\begin{equation}
    \underset{W}{\argmax} \quad \sum_{i,j} \Gamma_{i,j}e ^{- \frac{||W^Tr_i - W^Tr_j||^2}{2 \sigma^2}} \quad 
     s.t \quad W^TW = I.
     \label{eq:hsic_obj_with_gaussian2}
\end{equation}

Following Lemma~\ref{lemma:lemma1}, $\Gamma_{i,j}$ is positive if $(r_i,r_j)$ pair belongs to the same class, and it is negative when the pair are in different classes. We can split the summation into the positive and negative $\Gamma_{i,j}$ pairs.

\begin{equation}
    \underset{W}{\argmax} \quad \sum_{i,j \in S} \Gamma_{i,j}e ^{- \frac{||W^Tr_i - W^Tr_j||^2}{2 \sigma^2}} - \sum_{i,j \in S^c} \Gamma_{i,j}e ^{- \frac{||W^Tr_i - W^Tr_j||^2}{2 \sigma^2}}\quad 
     s.t \quad W^TW = I.
     \label{eq:hsic_obj_with_gaussian3}
\end{equation}
From Eq.~(\ref{eq:hsic_obj_with_gaussian3}), we see that given an appropriate $\sigma$ value the global optimal solution is achieved when the exponential terms are either 0 or 1 such that
\begin{equation}
    \underset{W}{\max} \quad \sum_{i,j \in S} \Gamma_{i,j}e ^{- \frac{||W^Tr_i - W^Tr_j||^2}{2 \sigma^2}} + \sum_{i,j \in S^c} -\Gamma_{i,j}e ^{- \frac{||W^Tr_i - W^Tr_j||^2}{2 \sigma^2}} = 
    \sum_{i,j \in S} \Gamma_{i,j}[1] - \sum_{i,j \in S^c} \Gamma_{i,j}[0]. 
     \label{eq:hsic_obj_with_gaussian4}
\end{equation}
Therefore, if there exists a $W^*$ that satisfies the following two conditions, $W^*$ must also be the global optimal. 
\begin{align}
    \label{eq:p23}
    \forall i,j \in S \quad & 
    \lim_{\sigma \rightarrow 0}
    e ^{- \frac{||W^Tr_i - W^Tr_j||^2}{2 \sigma^2}} = 1\\
    \label{eq:p24}
    \forall i,j \in S^c \quad & 
    \lim_{\sigma \rightarrow 0}
    e^{- \frac{||W^Tr_i - W^Tr_j||^2}{2 \sigma^2}} = 0.
\end{align}
Next, we consider the global optimal of the objective
\begin{equation}
    \underset{W}{\argmin} \quad
    \frac{1}{\sigma^2}
    \sum_{i,j \in \mathcal{S}} ||W^Tr_i - W^Tr_j||^2_{2} - 
    \frac{1}{\sigma^2}
    \sum_{i,j \in \mathcal{S}^c} ||W^Tr_i - W^Tr_j||^2_{2} 
    \quad \text{s.t : } \quad W^TW = I.
    \label{eq:dep_prop_obj}
\end{equation}
Similarly, we can state that if there exists a $W^*$ that satisfies the following two conditions, $W^*$ must also be the global optimal of Eq.~(\ref{eq:dep_prop_obj}).
\begin{align}
    \label{eq:pp2}
    \forall i,j \in S \quad & \lim_{\sigma \rightarrow 0}
        \frac{||W^Tr_i - W^Tr_j||^2}{2 \sigma^2} = 0\\
    \label{eq:pp3}
    \forall i,j \in S^c \quad & \lim_{\sigma \rightarrow 0} 
        \frac{||W^Tr_i - W^Tr_j||^2}{2 \sigma^2} = \infty.
\end{align}
Notice that the $W^*$ that satisfies conditions Eq.~(\ref{eq:pp2}) and (\ref{eq:pp3}) is the same $W^*$ that satisfies Eq.~(\ref{eq:p23}) and (\ref{eq:p24}). Therefore, if the global optimal of $W^*$ for Eq.~(\ref{eq:dep_prop_obj}) satisfies Eq.~(\ref{eq:pp2}) and (\ref{eq:pp3}), then the same $W^*$ would also be the global optimal for Eq.~(\ref{eq:hsic_obj_with_gaussian3}). 

Our goal is to use Eq.~(\ref{eq:hsic_obj_with_gaussian3}) as a surrogate to understand the conditions that guarantees the existence of $W^*$, thereby satisfying Eq.~(\ref{eq:pp2}) and (\ref{eq:pp3}). After, multiplying the square terms out, Eq.~(\ref{eq:dep_prop_obj}) becomes

\begin{equation}
    \underset{W}{\argmin} \quad
    \frac{1}{\sigma^2}
    \sum_{i,j \in \mathcal{S}} 
    (r_i - r_j)^T W W^T (r_i - r_j) - 
    \frac{1}{\sigma^2}
    \sum_{i,j \in \mathcal{S}^c} 
    (r_i - r_j)^T W W^T (r_i - r_j)
    \quad \text{s.t : } \quad W^TW = I.
    \label{eq:dep_prop_obj_2}
\end{equation}
Since $(r_i - r_j)^T W W^T (r_i - r_j)$ is a scalar value, we can place a Trace around the term and rotate them to obtain
\begin{equation}
    \underset{W}{\argmin} \quad
    \frac{1}{\sigma^2}
    \sum_{i,j \in \mathcal{S}} 
    \Tr[W^T (r_i - r_j)(r_i - r_j)^T W ] - 
    \frac{1}{\sigma^2}
    \sum_{i,j \in \mathcal{S}^c} 
    \Tr[W^T (r_i - r_j)(r_i - r_j)^T W]
    \quad \text{s.t : } \quad W^TW = I.
    \label{eq:dep_prop_obj_3}
\end{equation}
At this point, we can simply move the $\frac{1}{\sigma^2}$ value and the summation operation into the Trace to obtain
\begin{equation}
    \underset{W}{\argmin} \quad
    \Tr(W^T A_= W ) - 
    \Tr(W^T A_{\ne} W)
    \quad \text{s.t : } \quad W^TW = I.
    \label{eq:dep_prop_obj_4}
\end{equation}
%To push the Gaussian kernel to 1, we must minimize $||W^Tr_i - W^Tr_j||^2$ for $(i,j) \in \mathcal{S}$ towards 0 and maximize the same expression for pairs in $\bar{\mathcal{S}}$. Since $0 \le r_i^Tr_j \le 1$ and $W^TW=I$, $||W^Tr_i - W^Tr_j||$ is maximized at $\sqrt{2}$. Here, we observe that the same solution $W$ that minimizes Eq.~(\ref{eq:dep_prop_obj}) must also maximize Eq.~(\ref{eq:cov_objective2})
\end{proof}

\begin{lemma}\label{lemma:exist_weights}
    There exist a set of weights ${W_1, ..., W_L}$ such that the CCN objective generates a uniformly converging \textit{risk sequence}
\end{lemma}
\begin{proof}
Looking at the 1st term of Eq.~(\ref{eq:dep_prop_obj_3}) more carefully and focus on the $W^T (r_i - r_j)$ portion where $r_i$ and $r_j$ are assume to belong to the same class. In the most ideal case, we wish find a subspace projection $W$ that pulls all sample pairs together, i.e., we want $0 = W^T (r_i - r_j)$ for all $(r_i,r_j)$ pairs. This is possible only in the case where $W$ is in the null space of $A_=$.

Simultaneously, we want a $W$ that pushes $(r_i - r_j)$ distance infinitely large for the 2nd term. While infinity may not be possible, we know that the samples are maximally separated if $W$ is in the span of the eigenvectors of $A_{\ne}$ that has an associated positive eigenvalue. We refer to this set of eigenvectors as $V$. 

At this point, we can mentally draw the 2 spaces as 2 circles in a Venn diagram. One circle is the null space of $A_=$ while the other circle is the span of $V$. Therefore, the intersection of these 2 spaces would achieve both objectives simultaneously. Since the 1st term is pushed to 0, as long as the 2nd term is $\ne$ 0, we can set $\sigma$ to be very small to push the 2nd term toward infinity. Therefore, the key to the existence of $W^*$ is the existence of this intersection. Alternatively, we can state that if the null space of $A_=$ is sufficiently large such that it covers the span of $V$, then $W^*$ exists. 

Here, we leverage the feature map of a Gaussian kernel in that it has $A_= \in \mathbb{R}^{\infty \times \infty}$. Therefore, given that $A_=$ has a finite rank, its null space must have infinite dimensions. The only possibility for the null space of $A_=$ not to intersect with the span of $V$, is if $A_= = A_{\ne}$. Since $A_=$ and $A_{\ne}$ are by definition different, the null space of $A_=$ from a Gaussian kernel will always be sufficiently large to intersect the span of $V$, i.e., the usage of a Gaussian kernel guarantees the existence of $W^*$ for both Eq.~(\ref{eq:dep_prop_obj_4}) and (\ref{eq:hsic_obj_with_gaussian2}).

Given the existence of $W^*$ in the solution space of $\mathcal{W}$, we define its neighborhood of radius $r$ as 
\begin{equation}
    B_r(W^*) = \{W \in \mathcal{W}: d(W^*,W) < r\}.
\end{equation}
Given $B_r(W^*)$, there must also exist a $r$ and a set of $W$s, $\{W_1, ..., W^*\}$, sampled from interpolation points between a point within $B_r(W^*)$ and $W^*$ that monotonically improves the objective. In addition, since the Gaussian kernel is a Universal kernel, all of its functions in RKHS are continuous, therefore, the monotonic convergence is also uniform.
\end{proof}

We caution that proving the existence of a solution doesn't imply that the solution can be obtained easily or within a reasonable time. We have found experimentally that ISM is a fast algorithm that maintains this inequality with a uniform convergence.

\newpage 

\textbf{Aria's attempt:}

Define $\mathcal{E}_{l} = \{W^{*} = W_{1} ,\dots, W_{l}| W^{*} =      \underset{W}{\argmin} \quad
    \Tr(W^T A_= W ) - 
    \Tr(W^T A_{\ne} W)
    \quad \text{s.t : } \quad W^TW = I     \}$ to be the set of all weights that achieves optimal solution till depth $l$.
    
\textbf{Claim: The set $\mathcal{E}_{l} \subseteq (\mathcal{E}_{l+1})_{l}$ }.

If the claim is proven, the optimal solution at depth $l$ is consist of solutions at depth $l-1$, thus the optimal solution of depth $l$ is lower or equal than the optimal solution at depth $l-1$, meaning:

\begin{equation}
     ({\min} \quad
    \Tr(W^T A_= W ) - 
    \Tr(W^T A_{\ne} W)
    )_{l} \leq   ({\min} \quad
    \Tr(W^T A_= W ) - 
    \Tr(W^T A_{\ne} W)
    )_{l-1}
\end{equation}

Applying Lemma 2, we can conclude the following:
\begin{equation}
    \underset{f_l}{\max} \quad ||\text{Cov}(f_{l^\circ}(X), Y)||_F \geq
        ||\text{Cov}(f^*_{(l-1)^\circ}(X), Y)||_F.
\end{equation}

Hence the optimal $W$ for each depth induces a monotonically decreasing risk sequence. Furthermore the risk sequence is bounded from bellow by zero, thus the risk sequences is converging to its infimum.

\textbf{Proof of the claim}:

$\mathcal{E}_{l} \subseteq (\mathcal{E}_{l+1})_{l}$:

For proving the claim we prove the following:

$$W^{*} \in \mathcal{E}_{l} \rightarrow W^{*} \in \mathcal{E}_{l+1}$$

Assume $W^{*} \in \mathcal{E}_{l} $. Matrix $A_{=}, A_{\neq}$ is positive semi definite, hence, $\Tr(W^T A_= W ),\Tr(W^T A_{\neq}W)$ is always a positive number, thus if the optimal solution $W^{*}$ exists in depth $l$ should satisfies that $\Tr(W^T A_= W ) = 0$ and $\Tr(W^T A_{\neq} W ) \neq 0$.

\textbf{Studying the behavior of $\Tr(W^T A_= W ) = 0$}:

Again because $A_{=}$ is positive semi definite, $\Tr(W^T A_= W ) $ is only zero, if $ W^T A_= W   = \Vec{0}$, 

\begin{equation}
   W^T A_= W  = W^{T} \frac{1}{\sigma^2} \sum_{i,j \in \mathcal{S}} (r_i - r_j)(r_i - r_j)^T W =  \frac{1}{\sigma^2} \sum_{i,j \in \mathcal{S}} W^T (r_i - r_j)(r_i - r_j)^T W
\end{equation}
because every elements inside the summation $(r_i - r_j)(r_i - r_j)^T$ is positive semi definite matrix, hence, $W^T (r_i - r_j)(r_i - r_j)^T W = \Vec{0} , i,j \in \mathcal{S}$. Matrix $W$ can be seen through its columns $W = [W_{1},\dots,W_{q}]$, thus $W^T (r_i - r_j)(r_i - r_j)^T W = \Vec{0}$ becomes:

\begin{equation}
\begin{split}
    &W_{1}^T (r_i - r_j)(r_i - r_j)^T W_{1} = 0 = ||(r_i - r_j)^T W_{1}||_{2} = 0 \rightarrow (r_i - r_j)^T W_{1} = 0 \rightarrow r_i^{T} W_{1} = r_j^T W_{1}  
    \\
    .\\
    .\\
    .\\
   & W_{q}^T (r_i - r_j)(r_i - r_j)^T W_{q} = 0  = ||(r_i - r_j)^T W_{q}||_{2} = 0 \rightarrow (r_i - r_j)^T W_{q} = 0 \rightarrow r_i^{T} W_{q} = r_j^T W_{q}
    \end{split}
\end{equation}
Which means the in IDs space $r_{i}$ and $r_{j}$ get mapped to a same point through $W$ linear transformation for $i,j \in \mathcal{S}$.  

Assuming Gaussian feature map $\phi$, for $x_{i} = x_{j}$, after the nonlinear mapping, they mapped to the same point is RKHS space, meaning $\phi(x_{i}) = \phi(x_{j})$, and hence for the next depth $l+1$ adding any linear $W$ will still keep $i,j$ points on top of each other. Hence the We concluded that, if $W^{*} $ till layer $l$ satisfies $\Tr(W^T A_= W ) = 0$, adding any $W$ at layer $l+1$ will still keep this part of the objective the same.

\textbf{Studying the behavior of $\Tr(W^T A_{\neq} W ) >> 0$}:

With the same argument, we can use the fact that $A_{\neq}$ is semi positive definite, hence, $\Tr(W^T A_{\neq} W ) \neq 0$ is equivalent to $W^T A_{\neq} W  \neq \Vec{0}$, which means To be continued ...

 we know that $\phi$ is injective and hence based on definition of injectivity, we have:
 
 $$ x_{i} \neq x_{j} \rightarrow \phi(x_{i}) \neq \phi(x_{j}) $$
 
 which means if at layer $l$, the optimal $W^{*}$ does not map $i,j$ samples, after applying $\phi$, they are not going to map to each other, so at layer $l+1$ the samples not in the same class have distance, hence there exist a projection down keep this distances positive, \textbf{if point are distinct, is there a projection that keep their distance positive, I need to think to prove it but it makes sence, because if there, we don't really need it becuase of the following}, There exist a $W$ at step $l+1$, which still keeps them apart and that is W that all is zero and the second column is all one, due to the gaussian feature map, second the features map in second dimension in RKHS is invertable meaning, if $x_{i} \neq x_{j}$ then that elements is not equal as well, hence projection through that dimension keeps their distance. Hence choosing this $W$ for $l+1$, have all the criterias for optimal solution in $\mathcal{E}_{l+1}$.
 
 Hence every solution in $\mathcal{E}_{l}$ is inside the solution of $\mathcal{E}_{l+1}$.

 End of proof.

\textbf{Proving there exist a certain projection in Gaussian feature map that is injetive:}

Pick $W$ to be projection of the first two dimension of Gaussian kernel.
\textbf{Claim: $\phi \circ W$ is injective}

\textbf{proof}

\begin{equation}
\begin{split}
    X_{1}\exp{X_{1}^{2}} = X_{2}\exp{X_{2}^{2}}
    \\
    \exp{X_{1}^{2}} = \exp{X_{2}^{2}}
    \\
    \rightarrow X_{1} = X_{2}
    \end{split}
\end{equation}

\newpage

\textbf{Proof of global monotonically non-decreasing}:

\textbf{Claim}: \textit{There exists $W_{l}$, where $\mathcal{E}_{l-1}$ = $\mathcal{E}_{l}$}.

If the claim is proven, the optimal solution at depth $l$ is consist of solutions at depth $l-1$, thus the optimal solution of depth $l$ is lower or equal than the optimal solution at depth $l-1$, meaning:

\begin{equation}
     ({\min} \quad
    \Tr(W^T A_= W ) - 
    \Tr(W^T A_{\ne} W)
    )_{l} \leq   ({\min} \quad
    \Tr(W^T A_= W ) - 
    \Tr(W^T A_{\ne} W)
    )_{l-1}
\end{equation}

Applying Lemma 2, we can conclude the following:
\begin{equation}
    \underset{f_l}{\max} \quad ||\text{Cov}(f_{l^\circ}(X), Y)||_F \geq
        ||\text{Cov}(f^*_{(l-1)^\circ}(X), Y)||_F.
\end{equation}

Hence the optimal $W$ for each depth induces a monotonically decreasing risk sequence. Furthermore the risk sequence is bounded from bellow by zero, thus the risk sequences is converging to its infimum.

\textbf{Proof of the claim for the global case}:

For proving the claim we prove the following:

$$\exists W^{*} ,\,  \mathcal{E}_{l}(W_{1},\dots,W_{l-1},W^{*}) = \mathcal{E}_{l-1}(W_{1},\dots,W_{l-1})$$

Assume $W^{*} \in \mathcal{E}_{l} $. Matrix $A_{=}, A_{\neq}$ is positive semi definite, hence, $\Tr(W^T A_= W ),\Tr(W^T A_{\neq}W)$ is always a positive number, thus if the optimal solution $W^{*}$ exists in depth $l$ should satisfies that $\Tr(W^T A_= W ) = 0$ and $\Tr(W^T A_{\neq} W ) = \infty$.

\textbf{Studying the behavior of $\Tr(W^T A_= W ) = 0$}:
Again because $A_{=}$ is positive semi definite, $\Tr(W^T A_= W ) $ is only zero, if $ W^T A_= W   = \Vec{0}$, 

\begin{equation}
   W^T A_= W  = W^{T} \frac{1}{\sigma^2} \sum_{i,j \in \mathcal{S}} (r_i - r_j)(r_i - r_j)^T W =  \frac{1}{\sigma^2} \sum_{i,j \in \mathcal{S}} W^T (r_i - r_j)(r_i - r_j)^T W
\end{equation}
because every elements inside the summation $(r_i - r_j)(r_i - r_j)^T$ is positive semi definite matrix, hence, $W^T (r_i - r_j)(r_i - r_j)^T W = \Vec{0} , i,j \in \mathcal{S}$. Matrix $W$ can be seen through its columns $W = [W_{1},\dots,W_{q}]$, thus $W^T (r_i - r_j)(r_i - r_j)^T W = \Vec{0}$ becomes:

\begin{equation}
\begin{split}
    &W_{1}^T (r_i - r_j)(r_i - r_j)^T W_{1} = 0 \rightarrow W_{1}^T (r_i - r_j)(r_i - r_j)^T W_{1} W_{1}^{T} = 0 \rightarrow W_{1}^{T} A_{=}_{ij} = 0 \rightarrow A_{=}_{ij}^{T}W_{1} = A_{=}_{ij} W_{1} =0.
    \\
    .\\
    .\\
    .\\
   & W_{q}^T (r_i - r_j)(r_i - r_j)^T W_{q} = 0  = ||(r_i - r_j)^T W_{q}||_{2} = 0 \rightarrow (r_i - r_j)^T W_{q} = 0 \rightarrow r_i^{T} W_{q} = r_j^T W_{q}
    \end{split}
\end{equation}
Which means the in IDs space $r_{i}$ and $r_{j}$ get mapped to a same point through $W$ linear transformation for $i,j \in \mathcal{S}$.  

Assuming Gaussian feature map $\phi$, for $x_{i} = x_{j}$, after the nonlinear mapping, they mapped to the same point is RKHS space, meaning $\phi(x_{i}) = \phi(x_{j})$, and hence for the next depth $l+1$ adding any linear $W$ will still keep $i,j$ points on top of each other. Hence the We concluded that, if $W^{*} $ till layer $l$ satisfies $\Tr(W^T A_= W ) = 0$, adding any $W$ at layer $l+1$ will still keep this part of the objective the same.

\textbf{Studying the behavior of $\Tr(W^T A_{\neq} W ) >> 0$}:

With the same argument, we can use the fact that $A_{\neq}$ is semi positive definite, hence, $\Tr(W^T A_{\neq} W ) \neq 0$ is equivalent to $W^T A_{\neq} W  \neq \Vec{0}$, We can continue the same arguments and prove the following:

\begin{equation}
    W_{q}^T (r_i - r_j)(r_i - r_j)^T W_{q} >> 0 \rightarrow A_{\neq}_{ij} W_{q} >> 0 
\end{equation}

which corresponds to the largest eigenvalue.

 we know that $\phi$ is injective and hence based on definition of injectivity, we have:
 
 $$ x_{i} \neq x_{j} \rightarrow \phi(x_{i}) \neq \phi(x_{j}) $$
 
 which means if at layer $l$, the optimal $W^{*}$ does not map $i,j$ samples, after applying $\phi$, they are not going to map to each other, so at layer $l+1$ the samples not in the same class have distance, hence there exist a projection down keep this distances positive, There exist a $W$ at step $l$, which still keeps them apart and that is $W^{*} = [I_{q} 0]$, due to the gaussian feature map, as long as $q > 1$ we have a injective map, if $x_{i} \neq x_{j}$ then $\phi(x_{i}) \neq \phi(x_{j}) $, hence projection through that dimension keeps them distinct meaning in RKHS space composition of function till layer $l$ and after layer $l$ are geometrically equivalent, hence based on the corollary and theorem when $\simga \rightarrow \infty$, we have  $\mathcal{E}_{l} = \mathcal{E}_{l-1}$

 End of proof.

\textbf{Proving there exist a certain projection in Gaussian feature map that is injetive:}

Pick $W$ to be projection of the first two dimension of Gaussian kernel.
\textbf{Claim: $\phi \circ W$ is injective}

\textbf{proof}:

For $q>1$, we have the first two elements, hence:

\begin{equation}
\begin{split}
    X_{1}\exp{X_{1}^{2}} = X_{2}\exp{X_{2}^{2}}
    \\
    \exp{X_{1}^{2}} = \exp{X_{2}^{2}}
    \\
    \rightarrow X_{1} = X_{2}
    \end{split}
\end{equation}

\textbf{claim: The same proof works for local solution}

Picking $W_{l} = [I_{q},0]$, would makes $\phi \circ W_{l}$ injective. Hence if two points $x_{i}^{l-1}  \neq x_{j}^{l-1} $ then $\phi \circ W_{l}(x_{i}^{l-1} ) = x_{i}^{l}  \neq \phi \circ W_{l}(x_{j}^{l-1} ) = x_{j}^{l} $. Therefore the points samples that $x_{i}^{l-1}  = x_{j}^{l-1} $, we would have $\phi \circ W_{l}(x_{i}^{l-1} ) = \phi \circ W_{l}(x_{j}^{l-1} )$, and the point that are different would still be different. Hence 
\begin{align}
    \label{eq:p234}\forall x_{i}^{l-1} \neq x_{j}^{l-1}  \rightarrow r_{i} \neq r_{j} \rightarrow   ||W^Tr_i - W^Tr_j|| > 0  & 
    \rightarrow \lim_{\sigma \rightarrow 0}
    e ^{- \frac{||W^Tr_i - W^Tr_j||^2}{2 \sigma^2}} = 1\\
    \label{eq:p245}
    \forall x_{i}^{l-1}  = x_{j}^{l-1}  \rightarrow r_{i} = r_{j} \rightarrow   ||W^Tr_i - W^Tr_j|| = 0  & \rightarrow  
    \lim_{\sigma \rightarrow 0}
    e^{- \frac{||W^Tr_i - W^Tr_j||^2}{2 \sigma^2}} = 0.
\end{align}

%  \newpage

\newpage

\begin{definition}
Function $f,g : \mathbb{R}^{m} \rightarrow \mathbb{R}^{m}$ are geometrically equivalent iff:

\begin{equation}
    \forall x,y \in \mathbb{R}^{m}, d(f(x),f(y)) > 0 \Leftrightarrow  d(g(x),g(y))>0
\end{equation}

We show this, $f \approx_\textit{GE} g$
\end{definition}

\begin{theorem}
For function $W : \mathbb{R}^{m} \rightarrow \mathbb{R}^{m}$, if $W$ is injective: 

\begin{equation}
    W\circ f \approx_\textit{GE} f \approx_\textit{GE} f \circ W
\end{equation}

\end{theorem}
\begin{proof}
     \begin{equation}
   0 \sum_{i,j} \Gamma_{i,j}e ^{- \frac{||W^Tr_i - W^Tr_j||^2}{2 \sigma^2}} \quad 
     s.t \quad W^TW = I.
     \label{eq:proof help}
\end{equation}
\end{proof}

\begin{theorem} 
If $f \approx_\textit{GE} g$, $\forall \epsilon > 0$, $\exists \sigma_{0}$ which for $\forall \sigma \leq \sigma_{0}$ then:
\begin{equation}
|   || cov(f(x),Y)   ||_{F} - || cov(g(x),Y)   ||_{G} | \leq \epsilon
\end{equation}

\end{theorem}

\begin{corollary}
For injecive $W_{l}$,  $\exists \sigma_{0}$ which for $\forall \sigma \leq \sigma_{0}$ then:

$$ \epsilon_{l} \geq \epsilon_{l-1} $$
    
\end{corollary}

\begin{theorem}
Assume if: $|S^{c}| \geq 3$, then, $\forall i,j \in S$ 
$$Null(A_{ij}) \cap Span(A_{\neq}) \neq {0}$$
\end{theorem}

\begin{proof}

\textbf{Claim: $rank(A_{\neq}) > 1$}:

We prove this through contradiction. Assume  $rank(A_{\neq}) \leq 1$, so its either zero, or one. 

\begin{itemize}
    \item Case $rank(A_{\neq}) = 0$. We know that $A_{\neq} \geq 0$ hence, if the rank is zero, then $\forall  W \in \mathbb{R}^{m}$:

    \begin{equation}
        \begin{split}
        A_{\neq}W = \sum_{i} \phi_{i}\phi_{i}^{T}W \rightarrow 
        \\
        W^{T}A_{\neq}W = \sum_{i} W^{T}\phi_{i}\phi_{i}^{T}W \rightarrow W^{T}\phi_{i}\phi_{i}^{T}W = 0 \forall i
        \\  \rightarrow W = \phi_{i} \phi_{i}^{T}\phi_{i}\phi_{i}^{T}\phi_{i} = |\phi_{i}|^{2}= 0 \rightarrow
        \phi_{i} = 0 \forall i
        \end{split}
    \end{equation}

which is a contradiction because that means:

$$\forall i,j \in S^{c}, r_i = r_j$$, which means everything are just one point.
    
 \item Case $rank(A_{\neq}) = 1$.

 \begin{lemma}
     For $A = \sum_{i}^{n}  \phi_{i}\phi_{i}^{T}$, we have: 
     
     $$\textit{span}(A) = \textit{span}(\{\phi_{1},\dots,\phi_{n}\}) $$
     
\begin{proof}
     For any $W \in \mathbb{R}^{m}$ we have the following: 
     \begin{equation}
         A_{\neq} W= \sum_{i} \phi_{i}\phi_{i}^{T} W = \sum_{i} c_i \phi_{i}  
     \end{equation}
     where $c_{i} = \phi_{i}^{T} W$
\end{proof}     
     
 \end{lemma}
    
    Claim: Now Assuming $|S^{c}| \geq 3$, we have contradiction.
    
    assume the case $|S^{c}| = 3 $Choose three separate points from $S^{c}$, $r_{1},r_{2},r_{3}$ on the positive quarter of unit ball, without loss of generality assume choose $r_{1}$ to be the one with largest angle and $r_{3}$ with smallest. From previous lemma we know that span of $A_{\neq}$ is equal to $span \{(r_1 - r_2), (r_2 -r_3), (r_1-r_3)  \}$. having the condition that the rank is equal to one means that any vector $\{(r_1 - r_2), (r_2 -r_3), (r_1-r_3) \}$ can be represented as $\{(r_1 - r_3) \}$. In particular we have the following:
    
    \begin{equation}
    \begin{split}
        r_{1} - r_{2} =  \lambda_{1} (r_1 -r_3)
        \\
         r_{2} - r_{3} =  \lambda_{2} (r_1 -r_3)
    \end{split}
    \end{equation}
    
    Hence $r_{j} = r_{3}(1-\lambda_2) + \lambda_2 r_{1}$, because of the assumption that $r_{2}$ is between $r_{1}$ and $r_{3}$, hence we can assume $0<\lambda_2<1$. It is strict inequalities because the points are separate. Now we have the followings:
    
    \begin{equation}
    \begin{split}
        r_{2}^{T} r_{2} = ( r_{3}(1-\lambda_2) + \lambda_2 r_{1})^{T}( r_{3}(1-\lambda_2) + \lambda_2 r_{1}) 
        \\
         = 1 + 2\lambda_{2}^{2} - 2\lambda_2 + 2\lambda_2(1-\lambda_2) r_3^{T}r_{1} 
         \\ 
         < 1 + 2\lambda_{2}^{2} - 2\lambda_2 + 2\lambda_2(1-\lambda_2) = 1
    \end{split}
    \end{equation}

    which we used the fact that $ r_3^{T}r_{1}  < 1$ using the fact $r_{1} \neq r_3$. And $0<\lambda_2<1$. which is a contradiction due to the fact that the norm of $r_2$ is equal to one.

\end{itemize}

Hence this proves the claim that $rank(A_{\neq}) > 1$.

\begin{lemma}
    If $rank(A_{\neq}) > 1$ then, $\forall i,j \in S$:
    $$Null(A_{ij}) \cap Span(A_{\neq}) \neq \{0\}$$
\end{lemma}
    
    \begin{proof}
For $A_{ij} = (r_i-r_j)(r_i-r_j)^T$, hence it has a rank one, call the vector $r_i-r_j = \phi$. we have two cases 
\begin{itemize}
    \item $\phi\in span(A_{\neq})$: but the $span(A_{\neq})$ has more than element, hence other elements should be $null(A_{ij})$, hence $Null(A_{ij}) \cap Span(A_{\neq}) \neq \{0\}$. 
    \item $\phi\in null(A_{\neq})$, but the elements of $span(A_{\neq})$ should be in $null(A_{ij})$, hence $Null(A_{ij}) \cap Span(A_{\neq}) \neq \{0\}$. 
\end{itemize}       

So in either case the intersection is not empty.

    \end{proof}

This proves that for any elements $i,j \in S$, the intersection $Null(A_{ij}) \cap Span(A_{\neq}) \neq \{0\}$ has a non trivial element inside of it. 

\end{proof}

\begin{theorem}
For $|S^{c}| \geq 3$ then,$\exists W$, $\exists \sigma_{0}$ where $\forall \sigma \leq \sigma_{0}$ we have: 
    $$ \epsilon_{l} > \epsilon_{l-1} $$
\end{theorem}

\begin{proof}
     So
\end{proof}

\begin{corollary}
The global optimal solution can be reach in finite time solving greedy steps.
\end{corollary}

\end{appendices}

\newpage

\textbf{Aria's:}

\begin{theorem} For all $\sigma \leq \sigma_{0}$, $\exists W_{l}$
 
 \begin{equation}
    \underbrace{ 
    \sum_{i,j \in \mathcal{S}} \Gamma_{i,j} 
    e^{-\frac{(r_i-r_j)^TW_l W_l^T(r_i-r_j)}{2\sigma^2}}
    }_\text{1st term}
    -
    \underbrace{
    \sum_{i,j \in \mathcal{S}^c} \Gamma_{i,j} 
    e^{-\frac{(r_i-r_j)^TW_l W_l^T(r_i-r_j)}{2\sigma^2}} 
    }_\text{2nd term}
    \quad \geq \sum_{i,j \in \mathcal{S}\cup \mathcal{S}^{c}} \Gamma_{i,j} 
    r_{i}^{T}r_{j}
\end{equation}

\end{theorem}

\begin{proof}

Note that if any term from the last layer are mapped together, meaning $r_{i} = r_{j}$, then the LHS and RHS would be equal, so without loss of generality we can assume all the samples here are no equal, meaning $r_{i} \neq r_{j}$. For this proof assume we have two classes denoted as $\mathcal{S}^{1}, \mathcal{S}^{2}$.

\begin{lemma} For any $1>\mathcal{E} > 0$  ,$\exists \sigma_{0}$ that:

$$\forall i,j \quad r_{i}^Tr_{j} \leq \mathcal{E}$$

\end{lemma}

\begin{proof}

For previous kernel property, we know that:

$$<r_{i},r_{j}> = e^\frac{-|.|^2}{2\sigma ^2}$$
where $|.|$ is the distance before projecting to the RKHS space. We have finitely many of samples, hence there exists a maximum distance $|.|$ of them. Hence by choosing $\sigma_{0} = \sqrt{\frac{-|.|}{2\ln{\mathcal{E}}}}$, we conclude the proof of the lemma.

\end{proof}

Hence based on the lemma the upper bound of RHS is: 

\begin{equation}
    \sum_{i,j \in \mathcal{S}\cup \mathcal{S}^{c}} \Gamma_{i,j}
    r_{i}^{T}r_{j} \leq \mathcal{E} \sum_{i,j \in \mathcal{S}} \Gamma_{i,j} -  \sum_{i,j \in \cup \mathcal{S}^{c}} \Gamma_{i,j} \leq \mathcal{E} \sum_{i,j \in \mathcal{S}} \Gamma_{i,j}
\end{equation}

Hence we need to prove the following:

 \begin{equation}
    \underbrace{ 
    \sum_{i,j \in \mathcal{S}} \Gamma_{i,j} 
    e^{-\frac{(r_i-r_j)^TW_l W_l^T(r_i-r_j)}{2\sigma^2}}
    }_\text{1st term}
    -
    \underbrace{
    \sum_{i,j \in \mathcal{S}^c} \Gamma_{i,j} 
    e^{-\frac{(r_i-r_j)^TW_l W_l^T(r_i-r_j)}{2\sigma^2}} 
    }_\text{2nd term}
    \quad \geq \mathcal{E} \sum_{i,j \in \mathcal{S}} \Gamma_{i,j}
\end{equation}

\textbf{First term}:

By decreasing the $\sigma_{0}$, the $<r_{i},r_{j}>$ approaches to zero, meaning they become almost orthogonal.

hence there exist a finite orthogonal axis $\{e_{1},\dots, e_{n}\}$, where $n$ is the number of samples. and we have the following property:

\begin{lemma}
\begin{equation}
    \forall i,j <e_{i},r_{i}> \geq 1-\mathcal{E} , <e_{i},r_{j}> \leq \mathcal{E}.
\end{equation}
\end{lemma}

\begin{equation}
    \sum_{i,j \in \mathcal{S}} \Gamma_{i,j} 
    e^{-\frac{(r_i-r_j)^TW_l W_l^T(r_i-r_j)}{2\sigma^2}}
   = \sum_{i,j \in \mathcal{S}^1} \Gamma_{i,j} 
    e^{-\frac{(r_i-r_j)^TW_l W_l^T(r_i-r_j)}{2\sigma^2}}
   + \sum_{i,j \in \mathcal{S}^2} \Gamma_{i,j} 
    e^{-\frac{(r_i-r_j)^TW_l W_l^T(r_i-r_j)}{2\sigma^2}}
\end{equation}

pick $W =  \sum_{i\in \mathcal{S}^1}e_{i}$. Hence we have:

\begin{equation}
    \lim_{\mathcal{E} \longrightarrow 0}   \sum_{i,j \in \mathcal{S}^1} \Gamma_{i,j} 
    e^{-\frac{(r_i-r_j)^TW_l W_l^T(r_i-r_j)}{2\sigma^2}} = \sum_{i,j \in \mathcal{S}^1} \Gamma_{i,j} 
    e^{-\frac{2}{2\sigma^2}}
\end{equation}

and for $\mathcal{S}^2$:

\begin{equation}
    \lim_{\mathcal{E} \longrightarrow 0}   \sum_{i,j \in \mathcal{S}^2} \Gamma_{i,j} 
    e^{-\frac{(r_i-r_j)^TW_l W_l^T(r_i-r_j)}{2\sigma^2}} = \sum_{i,j \in \mathcal{S}^2} \Gamma_{i,j} 
    e^{-\frac{0}{2\sigma^2}} = \sum_{i,j \in \mathcal{S}^1} \Gamma_{i,j} 
\end{equation}

For $\mathcal{S}^c$

\begin{equation}
    \lim_{\mathcal{E} \longrightarrow 0}   \sum_{i,j \in \mathcal{S}^c} \Gamma_{i,j} 
    e^{-\frac{(r_i-r_j)^TW_l W_l^T(r_i-r_j)}{2\sigma^2}} = \sum_{i,j \in \mathcal{S}^c} \Gamma_{i,j} 
    e^{-\frac{1}{2\sigma^2}}
\end{equation}

\begin{lemma} We have the following:
\begin{equation}
    \sum_{i,j \in \mathcal{S}^1} \Gamma_{i,j} 
    e^{-\frac{2}{2\sigma^2}} + \sum_{i,j \in \mathcal{S}^1}  \Gamma_{i,j} - \sum_{i,j \in \mathcal{S}^c} \Gamma_{i,j} 
    e^{-\frac{1}{2\sigma^2}} \geq \mathcal{E} \sum_{i,j \in \mathcal{S}} \Gamma_{i,j}
\end{equation}

\end{lemma}
\begin{proof}

Taking things to one side would gives us the following: 

\begin{equation}
         \sum_{i,j \in \mathcal{S}^1}  \Gamma_{i,j} \geq \mathcal{E} \sum_{i,j \in \mathcal{S}} \Gamma_{i,j} -  \sum_{i,j \in \mathcal{S}^1} \Gamma_{i,j} 
    e^{-\frac{2}{2\sigma^2}} + \sum_{i,j \in \mathcal{S}^1}  + \sum_{i,j \in \mathcal{S}^c} \Gamma_{i,j} 
    e^{-\frac{1}{2\sigma^2}}
\end{equation}

The LHS is a positive number, and the RHS can be controlled to be arbitrary close to zero by making $\sigma$ of this layer and $\mathcal{E}$ small.  
\end{proof}

\begin{lemma}
    \begin{equation}
    \begin{split}
        \lim_{\mathcal{E} \longrightarrow 0}  ( \sum_{i,j \in \mathcal{S}^1} \Gamma_{i,j} 
    e^{-\frac{(r_i-r_j)^TW_l W_l^T(r_i-r_j)}{2\sigma^2}} +   &\sum_{i,j \in \mathcal{S}^c} \Gamma_{i,j} 
    e^{-\frac{(r_i-r_j)^TW_l W_l^T(r_i-r_j)}{2\sigma^2}} +   \sum_{i,j \in \mathcal{S}^c} \Gamma_{i,j} 
    e^{-\frac{(r_i-r_j)^TW_l W_l^T(r_i-r_j)}{2\sigma^2}} ) =
    \\
    &\sum_{i,j \in \mathcal{S}^1} \Gamma_{i,j} 
    e^{-\frac{2}{2\sigma^2}} + \sum_{i,j \in \mathcal{S}^2}  \Gamma_{i,j} - \sum_{i,j \in \mathcal{S}^c} \Gamma_{i,j} 
    e^{-\frac{1}{2\sigma^2}}
    \end{split}
    \end{equation}
    
    because every part of the RHS is continuous function of $\mathcal{E}$, hence we can get arbitrary close to the LHS.
    
\end{lemma}

Lets call the LHS of lemma 4 as $f_1$, ad RHS of it as $l_1$, and the RHS of lemma 3 as $l_2$.

We want to prove that $f_1 \geq l_2$. From lemma 3 we prove that we can make $f_1 - l_2> \delta >0$, in fact we make it as large as $ \sum_{i,j \in \mathcal{S}^2}  \Gamma_{i,j}$. From lemma 4 we know that we can make $|f_1-l_1|< \delta/3 $. hence we have $l_1 - l_2 > 2*\delta/3 > 0$. Hence the proof is compelte.

\end{proof}

\newpage
