# Supplementary material for: Kernel Dependence Network
Source: arXiv:2011.03320 source file (2020-11-09)
Supplement: Supplementary file 7 [file e_HSIC_as_CE.tex]

\begin{appendices}
\section{Proof for Corollary \ref{corollary:mse} and \ref{corollary:ce}}
\label{app:corollary:ce}

\textbf{Corollary} \ref{corollary:mse}: 
    \textit{Given $\hsic_l \rightarrow \hsic^*$, the network output in IDS solves MSE via a translation of labels.}
   
\begin{proof} \hspace{1pt}
\begin{adjustwidth}{0.5cm}{0.0cm}
    As $\hsic_l \rightarrow \hsic^*$, Thm.~\ref{thm:geometric_interpret} shows that sample of the same class are mapped into the same point. Assuming that $\fm$ has mapped the sample into $c$ points $\alpha = [\alpha_1, ..., \alpha_c]$ that's different from the truth label
    $\xi = [\xi_1, ..., \xi_c]$. Then the $\mse$ objective is minimized by translating the $\fm$ output by 
    \begin{equation}
        \xi - \alpha.
    \end{equation}
\end{adjustwidth}
\end{proof}

\textbf{Corollary} \ref{corollary:ce}: 
    \textit{Given $\hsic_l \rightarrow \hsic^*$, the network output in RKHS solves $\ce$ via a change of bases.}
    
\textbf{Assumptions, and Notations. }
\begin{enumerate}
    \item  
        $n $ is the number of samples.
    \item
        $\nclass$ is the number of classes.
    \item
        $y_i \in \mathbb{R}^{\nclass}$ is the ground truth label for the $i^{th}$ sample. It is one-hot encoded where only the $j^{th}$ element is 1 if $x_i$ belongs to the $j^{th}$ class, all other elements would be 0.
    \item
        We denote $\fm$ as the network, and $\hat{y}_i \in \mathbb{R}^{\nclass}$ as the network output where $\hat{y}_i = \fm(x_i)$. We also assume that $\hat{y}_i$ is constrained on a probability simplex where $1 = \hat{y}_i^T \mathbf{1}_n$.
    %\item
    %    We denote $\fm_{\hsic}$ as a network using $\hsic$ as the objective, and $\hat{z}_i \in \mathbb{R}^{\nclass}$ as the network output where $\hat{z}_i = \fm_{\hsic}(x_i)$. 
    %\item
    %    We denote the $j^{th}$ element of $z_i$, $y_i$, and $\hat{y}_i$ as $z_i$, $y_{i,j}$ and $\hat{y}_{i,j}$ respectively.
    \item
        We denote the $j^{th}$ element of $y_i$, and $\hat{y}_i$ as $y_{i,j}$ and $\hat{y}_{i,j}$ respectively.
    \item
        We define
    \begin{addmargin}[1em]{2em}% 1em left, 2em right
    \textbf{Orthogonality Condition: }
        A set of samples $\{\hat{y}_1, ..., \hat{y}_n\}$ satisfies the orthogonality condition if
        \begin{equation} 
        \begin{cases}
        \langle \hat{y_{i}}, \hat{y_{j}}\rangle =1 & \forall\quad i,j \textrm{ same class} \\
        \langle \hat{y_{i}}, \hat{y_{j}}\rangle=0 & \forall\quad i,j \textrm{ not in the same class}
        \end{cases}.
        \end{equation}
    \end{addmargin}
    \item
        We define the Cross-Entropy objective as 
        \begin{equation}
        \underset{\fm}{\argmin} -\sum_{i=1}^{n} \sum_{j=1}^{\nclass} y_{i,j} \log(\fm(x_{i})_{i,j}).
        \end{equation}
    \end{enumerate}
\begin{proof}\hspace{1pt}
\begin{adjustwidth}{0.5cm}{0.0cm}
From Thm.~\ref{thm:geometric_interpret}, we know that the network $\fm$ output, $\{ \hat{y}_1, \hat{y}_2, ..., \hat{y}_n \}$,  satisfy the orthogonality condition at $\hsic^*$. Then there exists a set of  orthogonal bases represented by $\Xi = [\xi_1, \xi_2, ..., \xi_c]$ that maps $\{ \hat{y}_1, \hat{y}_2, ..., \hat{y}_n \}$ to simulate the output of a softmax layer. Let $\xi_{i} = \hat{y}_{j} , j\in \cS^{i}$, i.e., for the $i_{th}$ class we arbitrary choose one of the samples from this class and assigns $\xi_i$ of that class to be equal to the sample's output. Realize in our problem we have $<\hat{y}_{i},\hat{y}_{i}> = 1$, so if $<\hat{y}_{i},\hat{y}_{j}> = 1$, then subtracting these two would lead to $<\hat{y}_{i},\hat{y}_{i}-\hat{y}_{j}> = 0$, which is the same as $\hat{y}_{i}=\hat{y}_{j}$.
So this representation is well-defined and its independent of choices of the sample from each group if they satisfy orthogonality condition.
Now we define transformed labels, $Y$ as:
\begin{equation}
    Y = \hat{Y} \Xi.
\end{equation}
Note that $Y = [y_1, y_2, ..., y_n]^T$ which each $y_{i}$ is a one hot vector representing the class membership of $i$ sample in $c$ classes.
Since given $\Xi$ as the change of basis, we can match $\hat{Y}$ to $Y$ exactly, $\ce$ is minimized.
\end{adjustwidth}
\end{proof}
\end{appendices}
