# Supplementary material for: Kernel Dependence Network
Source: arXiv:2011.03320 source file (2020-11-09)
Supplement: Supplementary file 8 [file e_app_5.tex]

\begin{appendices}
\section{KNet's Relationship to Information Bottleneck}
\label{app:theorem_information_bottleneck}

Representing a layer from the HSIC perspective is descriptive of its objective mechanically. Namely, it can be visualized that it is finding the weights $W_l$ to map into the IDS such that when it is mapped back to RKHS, the new representation possesses a maximal dependence on the labels. While this understanding explains the network process mechanically, there also exists a strong relationship to information theory. 

Here, let $P(X)$ and $P(Y)$ be the probability distribution for samples for $X$ and $Y$. From statistics, besides the correlation index, dependence can also be measured by the distance between $P(X)P(Y)$ to $P(X,Y)$, where a distance of 0 implies a complete independence between $X$ and $Y$. In information theory, this dependence is measured by the Mutual Information (MI) where the distance between $P(X)P(Y)$ to $P(X,Y)$ is measured by KL divergence. Therefore, when the mutual information between $X$ and $Y$ is maximized, the statistical dependence between $P(X)$ and $P(Y)$ is also maximized. 

HSIC is related to MI in that it also measures the distances between $P(X)P(Y)$ and $P(X,Y)$. However, instead of using KL divergence, HSIC uses a metric called Maximal Mean discrepancy (MMD). Therefore, when we maximize the HSIC of a layer output to its labels, we are simultaneously discovering a mapping where the distribution of its images is highly dependent on the labels. 

By establishing the relationship between HSIC and MI, an MLP using Eq.~(\ref{eq:hsic_obj_pure}) can be interpreted as an information bottleneck (IB) defined by \citet{tishby2000information}, i.e., the network compresses the data while filtering out information unrelated to the labels. Here, we provide a short proof of this relationship.

\begin{proof}
\citet{tishby2000information} defined relevant information in signal $x \in X$ as being the information that this signal provides about another signal $y \in Y$. The information bottleneck concept compresses $x$ into $\hat{x}$ such that $\hat{x}$'s information about $y$ is maximally retained. They measure this minimally sufficient amount of information through the information bottleneck formulation where they maximize

\begin{equation}
    \underset{\hat{X}}{\max} \quad MI(\hat{X}, Y) - \beta MI(\hat{X}, X). 
     \label{eq:information_bottleneck}
\end{equation}

Since HSIC also measure the distance between distributions, by changing KL divergence to MMD, each layer can be defined by the same information bottleneck rewritten into 

\begin{equation}
    \underset{W}{\max} \quad HSIC(R_{l-1}W, Y) - \beta HSIC(R_{l-1}W, R_{l-1}),
     \label{eq:HSIC_information_bottleneck}
\end{equation}

or

\begin{equation}
    \underset{W}{\max} 
    \hspace{0.2cm}
    \Tr(K_{R_{l-1}W} HK_YH) - \beta \Tr(K_{R_{l-1}W} H K_{R_{i}}H).
\end{equation}

Applying the property of trace to sum two terms, it then becomes 

\begin{equation}
    \underset{W}{\max} 
    \hspace{0.2cm}
    \Tr(K_{R_{l-1}W} H(K_Y-\beta K_{R_{i}})H).
\end{equation}

We next take the Cholesky decomposition and get $\hat{Y} \hat{Y}^T = H(K_Y-\beta K_{R_{i}})H$, the formulation again reduces down to the proposed HSIC formulation of 

\begin{equation}
    \underset{W}{\max} 
    \hspace{0.2cm}
    HSIC(R_{l-1}W, \hat{Y}),
\end{equation}

where the definition of a label $\hat{Y}$ now includes the input information. This suggests that by adjusting the label definition of the HSIC formulation, MLP acts as a information bottleneck if the distances between distributions are measured by MMD.

\end{proof}
\end{appendices}
