# Supplementary material for: Kernel Dependence Network
Source: arXiv:2011.03320 source file (2020-11-09)
Supplement: Supplementary file 9 [file f_HSIC_as_MSE.tex]

\begin{appendices}
\section{Proof for Theorem \ref{thm:HSIC_as_MSE}}
\label{app:theorem_3_proof}
\textbf{Theorem} \ref{thm:HSIC_as_MSE}
\textit{The argmin of the MSE objective is satisfied by the argmax of the HSIC objective if the final $\Psi$ is discarded to produce an output in IDS.} 

\subsection{Assumptions and Notations of the Proof}
Given $\mathcal{S}$ and $\mathcal{S}^c$ as sets of all pairs of samples of $(x_i,x_j)$ from a dataset $X$ that belongs to the same and different classes respectively. We let $c$ be the number of classes and let $\Gamma_{i,j}$ be a set of  scalars derived from the labels following Lemma~\ref{lemma:lemma1}.

We prove this theorem by breaking the proof into three lemmas. 
Previously in Appendix~\ref{app:theorem_2_proof}, we have denoted $\hat{y}_i$ as the output of a layer after the activation function. We have specifically emphasized that $\hat{y}_i$ resides within RKHS. Here we denote the output of a layer for $x_i$ as $\hat{z}_i$  where the output is the point after the linear transformation $W$ \textit{prior} to the activation function, i.e., $W^T x_i = \hat{z}_i$. Therefore, although we are looking at the same formulation, we now focus on what is happening within IDS as HSIC is being optimized. Following this notation, we denote $z_i$ as the ground truth label for the sample $x_i$. 

\subsection{Summary the Proof}
To summarize the proof, we first prove in Lemma~\ref{lemma:mse_min_condition} that the MSE is minimized if and only if 

\[
\ \begin{cases}
 (\hat{z_{i}} - \hat{z_{j}})^2 = 0 & \textrm{if}\quad i,j \textrm{ same class} \\
 (\hat{z_{i}} - \hat{z_{j}})^2 \ne 0  & \textrm{if}\quad i,j \textrm{ not in the same class}
\end{cases}.
\]

In Lemma~\ref{lemma:HSIC_mse_opt_condition}, we show that that the HSIC objective using a Gaussian kernel is optimized if and only if  

\[
\ \begin{cases}
 (\hat{z_{i}} - \hat{z_{j}})^2 = 0 & \textrm{if}\quad i,j \textrm{ same class} \\
 (\hat{z_{i}} - \hat{z_{j}})^2 = 2& \textrm{if}\quad i,j \textrm{ not in the same class}
\end{cases}.
\]

Finally, in Lemma~\ref{lemma:HSIC_satisfies_MSE}, we draw from Lemma~\ref{lemma:mse_min_condition} and \ref{lemma:HSIC_mse_opt_condition} to show since the solutions space using the HSIC objective is a subset within the solution space using MSE, a solution that solves the HSIC objective must also satisfy MSE.

\subsection{Lemmas of the Proof}
\begin{lemma}\label{lemma:mse_min_condition}
The MSE is minimized if and only if 

\[
\ \begin{cases}
 (\hat{z_{i}} - \hat{z_{j}})^2 = 0 & \textrm{if}\quad i,j \textrm{ same class} \\
 (\hat{z_{i}} - \hat{z_{j}})^2 \ne 0  & \textrm{if}\quad i,j \textrm{ not in the same class}
\end{cases}.
\]
\end{lemma}

\begin{proof}
First, we assume that the MSE objective is already optimized, this implies that the output must satisfy $\hat{z}_i = z_i$ for any sample. Since $z_i = z_j$ for all samples of the same class, the condition $\hat{z}_i = \hat{z}_j$ must also be satisfied. As for the 2nd condition of $(\hat{z_{i}} - \hat{z_{j}})^2 \ne 0$ when $i,j$ are not in the same class, this is immediately satisfied by the definition of classification by MSE. 

Conversely, we next assume that $(\hat{z_{i}} - \hat{z_{j}})^2 = 0$ if sample pair $(x_i, x_j)$ are in the same class, and $(\hat{z_{i}} - \hat{z_{j}})^2 \neq 0$ if they are in different classes. This implies that all samples are mapped onto $c$ distinct points. Since MSE is a supervised problem, the labels can then be easily matched to one of the $c$ distinct points such that for each sample $\hat{z}_i$ we get $z_i = \hat{z}_i$. From here, it can be easily seen that the MSE objective is minimized to 0.

\begin{equation}
    0 = \sum_{i,j \in \mathcal{S}} (z_i - \hat{z}_i)^2 
\end{equation}
\end{proof}

\begin{lemma}\label{lemma:HSIC_mse_opt_condition}
The HSIC objective is optimized if and only if 

\[
\ \begin{cases}
 (\hat{z_{i}} - \hat{z_{j}})^2 = 0 & \textrm{if}\quad i,j \textrm{ same class} \\
 (\hat{z_{i}} - \hat{z_{j}})^2 = 2 & \textrm{if}\quad i,j \textrm{ not in the same class}
\end{cases}.
\]
\end{lemma}

\begin{proof}
First we assume that the HSIC objective using a Gaussian kernel is already optimized. This yields the optimal parameters for the MLP where

\begin{equation}
    \theta^* = 
    \underset{\theta}{\argmax} \quad \sum_{i,j} \Gamma_{i,j}e ^{-\gamma||g_\theta(x_i) - g_\theta(x_j)||^2}. 
     \label{eq_app:hsic_obj_with_gaussian_4}
\end{equation}

Applying Lemma~\ref{lemma:lemma1}, when $\Gamma_{i,j} > 0$  
the objective is maximized when $g_\theta$ forces $||g_\theta(x_i) - g_\theta(x_j)||^2$ towards 0. Conversely, when $\Gamma_{i,j} < 0$, $g_\theta$ will push $||g_\theta(x_i) - g_\theta(x_j)||$ towards the diameter of the solutions space. Here, by using the Gaussian kernel, we know that the maximum distance between two unit vectors is $\sqrt{2}$. By appropriately setting $\gamma$, we can ensure that 
\begin{equation}
    e^{-2\gamma } \approx 0.
\end{equation}

Converse, if we assume that $(\hat{z_{i}} - \hat{z_{j}})^2 = 0$ for all $(x_i,x_j)$ sample pairs in the same class and $(\hat{z_{i}} - \hat{z_{j}})^2 = \sqrt{2}$ for samples from different classes, if we plug these conditions into Eq.~(\ref{eq_app:hsic_obj_with_gaussian_4}) then
\begin{equation}
    \sum_{i,j \in \mathcal{S}} \Gamma_{i,j} = 
    \underset{\theta}{\max} \quad \sum_{i,j} \Gamma_{i,j}e ^{-\gamma(g_\theta(x_i) - g_\theta(x_j))^2}. 
     \label{eq_app:hsic_obj_with_gaussian_6}
\end{equation}
 
 Since $\sum_{i,j \in \mathcal{S}} \Gamma_{i,j}$ is the absolute upper bound for Eq.~(\ref{eq_app:hsic_obj_with_gaussian_6}), this solution must also be the optimal. 
 
\end{proof}

\begin{lemma}\label{lemma:HSIC_satisfies_MSE}
The the optimal condition of the MSE objective is satisfied if the HSIC objective is optimized.
\end{lemma}

\begin{proof}
When solving MSE, the labels can be anywhere. As long as different labels are distinguishable from each other, the distance between samples of different classes is not part of the objective. 

For HSIC since the distance between samples is part of the objective, the labels must be exactly $\sqrt{2}$ apart at an optimal solution. Therefore, the HSIC solution is a specific case of the MSE solution space.

We let the argmin solution space of MSE be $\mathcal{M}$ and the argmax solution space of HSIC be $\mathcal{H}$, then $\mathcal{H} \subset \mathcal{M}$. Therefore, a solution within $\mathcal{H}$ must also be a solution within $\mathcal{M}$. Which lead us to conclude that the argmax of the HSIC objective must also satisfy the MSE objective. 
\end{proof}
\end{appendices}
