# Supplementary material for: Kernel Dependence Network
Source: arXiv:2011.03320 source file (2020-11-09)
Supplement: Supplementary file 10 [file g_properties.tex]

\begin{appendices}
\section{Proof for Property \ref{prop:pulling_samples_together}}
\label{app:optimizing_IDS}

\begin{proof}
Given $\Gamma = HYY^TH$ and assuming that we use the traditional Gaussian kernel for $\Psi$, then at each layer, the objective becomes 
\begin{equation}
    \underset{W}{\max} \quad \sum_{i,j} \Gamma_{i,j}e ^{-\gamma(W^Tx_i - W^Tx_j)^2} \hspace{0.2cm}
     \text{s.t} \hspace{0.2cm} W^TW = I.
     \label{eq:hsic_obj_with_gaussian_2}
\end{equation}
By applying Lemma~\ref{lemma:lemma1}, the HSIC objective is maximized when $(W^Tx_i - W^Tx_j)=0$ for all $(x_i,x_j)$ samples of the same class, and $(W^Tx_i - W^Tx_j)$ is maximized for pairs in different classes. Notice that these results come after applying the input by $W$, therefore, these observations are happening in the IDS.
\end{proof}
\end{appendices}

\begin{appendices}
\section{Proof for Property \ref{prop:align_samples_together}}
\label{app:optimizing_RKHS}
\begin{proof}
We first note that Eq.~(\ref{eq:hsic_obj_with_gaussian_2}) can also be written as 
\begin{equation}
    \underset{W}{\max} \quad \sum_{i,j} \Gamma_{i,j} \langle 
    \psi(W^Tx_i), \psi(W^T x_j) \rangle, 
     \hspace{0.2cm} \text{s.t} \hspace{0.2cm} W^TW = I.
     \label{eq:hsic_obj}
\end{equation}
Assuming the conditions defined in Lemma~\ref{lemma:lemma1}, HSIC is optimized when the angular distance is pushed towards 0 and $\pi/2$.  Therefore, the Gaussian kernel pushes samples to become perfectly aligned or orthogonal on a unit hypersphere in RKHS. 
\end{proof}
\end{appendices}

%\begin{appendices}
%\section{Example of Using the Polynomial Kernel}
%\label{app:using_polynomial_kernel}
%\begin{proof}
%Using the polynomial kernel, the HSIC objective can be rewritten as 
%\begin{equation}
%    \underset{W}{\max} \quad \sum_{i,j} \Gamma_{i,j} (x_i^TW W^Ty_j + 1)^2. 
%     \label{eq:hsic_obj_with_poly}
%\end{equation}
%Following the same logic from the Gaussian kernel, we see that when two samples are in the same class, the optimal $W_l$ for the polynomial kernel pushes samples to be angularly aligned. However, when the samples are in different classes, $W_l$ will push the samples to points in opposite directions. Therefore, the polynomial kernel uses angular distance as the metric in IDS. This points to an interesting observation. Namely, that the kernel function defines the metric of similarity in IDS. However, once the samples are projected into RKHS, the inner product is always used as the metric. 
%\end{proof}
%\end{appendices}
