# Supplementary material for: Kernel Dependence Network
Source: arXiv:2011.03320 source file (2020-11-09)
Supplement: Supplementary file 11 [file i_app_9.tex]

\begin{appendices}
\section{ISM Algorithm}
\label{app:ISM Algorithm}

To define $\Phi$, we must first define $\Psi$ and $\mathcal{L}_\Psi$. If we let $\odot$ be the Hadamard product between matrices, then $\Psi = \Gamma \odot K_{XW}$. Given $\Psi$, we define $D_\Psi$ and $\mathcal{L}_{\Psi}$ respectively as the degree matrix and the Laplacian of $\Psi$ where $D_\Psi=\text{Diag}(\Psi 1_n)$ and $\mathcal{L}_\Psi = D_\Psi - \Psi$. Having the key notations defined, the $\Phi$ matrix associated with the Gaussian kernel is defined as
    \begin{equation}
        \Phi=-X^T\mathcal{L}_{\Psi} X.
        \label{eq:def_phi}
    \end{equation}
Since $\Phi$ associated with the Gaussian kernel is itself a function of $W$, an approximation of $\Phi$ via the 2nd order Taylor expansion produces an $\Phi_0$ independent of $W$ defined as
    \begin{equation}
        \Phi_0=-X^T \mathcal{L}_{\Gamma} X.
    \end{equation}
Since the Laplacian matrix based on $\Gamma$ no longer require $W$, an initial $W_0$ can be used 
for Eq.~(\ref{eq:def_phi}) to obtain $W_1$. By follow this pattern, ISM iteratively use $W_i$ to find $W_{i+1}$ until convergence. While this work focuses on the Gaussian kernel, we include the $\Phi/\Phi_0$ equation for other kernels in Tables~\ref{table:init_phis} and \ref{table:phis}. The ISM algorithm is also included in Algorithm~\ref{alg:ism}.

For convergence, we can converge when the Frobenius Norm $||W_i - W_{i-1}||_F$ falls below a predefined threshold $\delta$. However, based on the ISM algorithm, they found that in practice, the comparison of the most dominant eigenvalues is faster.

\begin{table}[h]   
\begin{minipage}{2.4in}
    \footnotesize
      \begin{tabular}{c|l}
        Kernel & Approximation of $\Phi$s\\
        \midrule
            Linear
            	& $\Phi_0=X^T\Gamma X$ \\
            Squared
            	& $\Phi_0=X^T \mathcal{L}_{\Gamma} X$ \\  
            Polynomial
            	& $\Phi_0=X^T \Gamma X$\\
            Gaussian
            	& $\Phi_0=-X^T \mathcal{L}_{\Gamma} X$\\
            Multiquadratic
            	& $\Phi_0=X^T\mathcal{L}_{\Gamma} X$\\
            \bottomrule       
      \end{tabular}
      \caption{Equations for the approximate \\$\Phi$s for the common kernels.}
      \label{table:init_phis}
\end{minipage}
\begin{minipage}{2in}
    \footnotesize
      \begin{tabular}{c|l}
        Kernel & $\Phi$ Equations\\
        \midrule
            Linear
            	& $\Phi=X^T\Gamma X$ \\
            Squared
            	& $\Phi=X^T \mathcal{L}_{\Gamma}X$ \\  
            Polynomial
            	& $\Phi=X^T\Psi X$ 
             	\hspace{0.2cm}
            	,
            	\hspace{0.2cm}           	
            	$\Psi = \Gamma \odot K_{XW,p-1}$ \\ 
            Gaussian
            	& $\Phi=-X^T\mathcal{L}_{\Psi} X$ 
            	,
            	$\Psi = \Gamma \odot K_{XW}$\\
            Multiquadratic
            	& $\Phi=X^T\mathcal{L}_{\Psi} X$ 
            	,
            	$\Psi = \Gamma \odot K_{XW}^{(-1)}$\\ 
        \bottomrule       
      \end{tabular}
      \caption{Equations for $\Phi$s for the common kernels.}
      \label{table:phis}
\end{minipage}
\end{table}

%\begin{table}[h]   
%    \centering
%      \begin{tabular}{c|l}
%        Kernel & Approximation of $\Phi$s\\
%        \midrule
%            Linear
%            	& $\Phi_0=X^T\Gamma X$ \\
%            Squared
%            	& $\Phi_0=X^T \mathcal{L}_{\Gamma} X$ \\  
%            Polynomial
%            	& $\Phi_0=X^T \Gamma X$\\
%            Gaussian
%            	& $\Phi_0=-X^T \mathcal{L}_{\Gamma} X$\\
%            Multiquadratic
%            	& $\Phi_0=X^T\mathcal{L}_{\Gamma} X$\\
%            \bottomrule       
%      \end{tabular}
%      \caption{Equations for approximate $\Phi$s for the common kernels.}
%      \label{table:init_phis}
%\end{table}
%
%\begin{table}[h]
%    \centering
%    \begin{tabular}{c|l}
%      Kernel & $\Phi$ Equations\\
%      \midrule
%          Linear
%          	& $\Phi=X^T\Gamma X$ \\
%          Squared
%          	& $\Phi=X^T \mathcal{L}_{\Gamma}X$ \\  
%          Polynomial
%          	& $\Phi=X^T\Psi X$ 
%           	\hspace{0.2cm}
%          	,
%          	\hspace{0.2cm}           	
%          	$\Psi = \Gamma \odot K_{XW,p-1}$ \\ 
%          Gaussian
%          	& $\Phi=-X^T\mathcal{L}_{\Psi} X$ 
%          	,
%          	$\Psi = \Gamma \odot K_{XW}$\\
%          Multiquadratic
%          	& $\Phi=X^T\mathcal{L}_{\Psi} X$ 
%          	,
%          	$\Psi = \Gamma \odot K_{XW}^{(-1)}$\\ 
%      \bottomrule       
%    \end{tabular}
%    \caption{Equations for $\Phi$s for the common kernels.}
%    \label{table:phis}
%\end{table}

    \begin{algorithm}[H]
    \footnotesize
     \textbf{Input :} Data $X$, kernel, Subspace Dimension $q$\\ \textbf{Output :} Projected subspace $W$ \\
     \textbf{Initialization :} Initialize $\Phi_0$ using Table~\ref{table:init_phis}.\\ Set $W_0$ to $V_{\text{max}}$ of $\Phi_0$.\\
     \While{$||\Lambda_i - \Lambda_{i-1}||_2/||\Lambda_i||_2 < \delta$ }{
        Compute $\Phi$ using Table~\ref{table:phis}\\
        Set $W_k$ to $V_{\text{max}}$ of $\Phi$
     }
     \caption{ISM Algorithm}
     \label{alg:ism}
    \end{algorithm}    

\end{appendices}
