# Supplementary material for: Kernel Dependence Network
Source: arXiv:2011.03320 source file (2020-11-09)
Supplement: Supplementary file 12 [file j_app_a_dataset.tex]

\newpage
\begin{appendices}
\section{Dataset Details}
\label{app:data_detail}

No samples were excludes from any of the dataset. 

\textbf{Wine. } 
    This dataset has 13 features, 178 samples, and 3 classes. The features are continuous and heavily unbalanced in magnitude. The dataset can be downloaded at \url{https://archive.ics.uci.edu/ml/datasets/wine.}

 \textbf{Divorce. } 
    This dataset has 54 features, 170 samples, and 2 classes. The features are discrete and balanced in magnitude.  The dataset can be downloaded at \url{https://archive.ics.uci.edu/ml/datasets/Divorce+Predictors+data+set.}
    
 \textbf{Car. } 
     This dataset has 6 features, 1728 samples and 2 classes. The features are discrete and balanced in magnitude.  The dataset can be downloaded at \url{https://archive.ics.uci.edu/ml/datasets/Car+Evaluation.}       
 
\textbf{Cancer. } 
    This dataset has 9 features, 683 samples, and 2 classes. The features are discrete and unbalanced in magnitude. The dataset can be downloaded at \url{https://archive.ics.uci.edu/ml/datasets/Breast+Cancer+Wisconsin+(Diagnostic)}.
    
 \textbf{Face. } 
    This dataset consists of images of 20 people in various poses. The 624 images are vectorized into 960 features.  
    The dataset can be downloaded at 
    \url{https://archive.ics.uci.edu/ml/datasets/CMU+Face+Images}.

\textbf{Random. } 
    This dataset has 2 features, 80 samples and 2 classes. It is generate with a gaussian distribution where half of the samples are randomly labeled as 1 or 0.
    
\textbf{Adversarial. } 
    This dataset has 2 features, 80 samples and 2 classes. It is generate with the following code:
    \begin{lstlisting}    
    #!/usr/bin/env python
    
    n = 40
    X1 = np.random.rand(n,2)
    X2 = X1 + 0.01*np.random.randn(n,2)
    
    X = np.vstack((X1,X2))
    Y = np.vstack(( np.zeros((n,1)), np.ones((n,1)) ))
    \end{lstlisting}    
 
\end{appendices}
