# Supplementary material for: Kernel Dependence Network
Source: arXiv:2011.03320 source file (2020-11-09)
Supplement: Supplementary file 13 [file k_metrics.tex]

%\begin{appendices}
%\section{Equations for Evaluation Metrics}
%\label{app:metric_calculation}
%For all metrics assume that $X \in \mathbb{R}^{n \times d}$ and $Y \in \mathbb{R}^{n \times c}$ as the data and the label respectively. 
%
%\textbf{Normalized HSIC. } 
%    The normalized HSIC can be calculated with 
%    \begin{equation}
%        \mathbb{H} = \frac{HSIC(X,Y)}{\sqrt{HSIC(X,X) HSIC(Y,Y)}}.
%    \end{equation}    
%
%\textbf{Silhouette Score. } 
%    We used the Silhouette score library from Sklearn with the function \url{https://scikit-learn.org/stable/modules/generated/sklearn.metrics.silhouette_score.html}.
%    The Silhouette Coefficient is calculated using the mean intra-cluster distance (a) and the mean nearest-cluster distance (b) for each sample. The Silhouette Coefficient for a sample is (b - a) / max(a, b). To clarify, b is the distance between a sample and the nearest cluster that the sample is not a part of. 
%    
%\textbf{Average Cosine Similarity Ratio (CS). } 
%    Given $\mathcal{S}$ and $\mathcal{S}^c$ as sets of all pairs of samples of $(x_i,x_j)$ from a dataset $X$ that belongs to the same and different classes respectively. The average cosine similarity ratio is defined as 
%    \begin{equation}
%    CS = \frac
%    {\sum_{i,j \in \mathcal{S}^c} \langle f(x_i), f(x_j) \rangle}
%    {\sum_{i,j \in \mathcal{S}} \langle f(x_i), f(x_j) \rangle}.
%    \end{equation}
%    Since the inner product between samples not in the same class should be 0, this ratio should approach 0 as the ratio improves.
%\end{appendices}

\begin{appendices}
%\section{\texorpdfstring{$W_l$} Dimensions for each 10 Fold of each Dataset}
\section{$W_l$ Dimensions for each 10 Fold of each Dataset}
\label{app:W_dimensions}
We report the input and output dimensions of each $W_l$ for every layer of each dataset in the form of $(\alpha, \beta)$; the corresponding dimension becomes $W_l \in \mathbb{R}^{\alpha \times \beta}$. Since each dataset consists of 10-folds, the network structure for each fold is reported. We note that the input of the 1st layer is the dimension of the original data. However, after the first layer, the width of the RFF becomes the output of each layer; here we use 300. 

The $\beta$ value is chosen during the ISM algorithm. By keeping only the most dominant eigenvector of the $\Phi$ matrix, the output dimension of each layer corresponds with the rank of $\Phi$. It can be seen from each dataset that the first layer significantly expands the rank. The expansion is generally followed by a compression of fewer and fewer eigenvalues. These results conform with the observations made by \citet{montavon2011kernel} and \citet{ansuini2019intrinsic}.

\begin{tabular}{ll}
\centering
\tiny
\setlength{\tabcolsep}{7.0pt}

\begin{tabular}{cccccc|}
	\hline
Data & Layer 1 & Layer 2 & Layer 3 & Layer 4 \\ 
	\hline
adversarial 1 & (2, 2) & (300, 61) & (300, 35) \\ 
adversarial 2 & (2, 2) & (300, 61) & (300, 35) \\ 
adversarial 3 & (2, 2) & (300, 61) & (300, 8) & (300, 4) \\ 
adversarial 4 & (2, 2) & (300, 61) & (300, 29) \\ 
adversarial 5 & (2, 2) & (300, 61) & (300, 29) \\ 
adversarial 6 & (2, 2) & (300, 61) & (300, 7) & (300, 4) \\ 
adversarial 7 & (2, 2) & (300, 61) & (300, 34) \\ 
adversarial 8 & (2, 2) & (300, 12) & (300, 61) & (300, 30) \\ 
adversarial 9 & (2, 2) & (300, 61) & (300, 33) \\ 
adversarial 10 & (2, 2) & (300, 61) & (300, 33) \\ 
	\hline
\end{tabular}
&
\centering
\tiny
\setlength{\tabcolsep}{3.0pt}

\begin{tabular}{ccccc|}
	\hline
Data & Layer 1 & Layer 2 & Layer 3 \\ 
	\hline
Random 1 & (3, 3) & (300, 47) & (300, 25) \\ 
Random 2 & (3, 3) & (300, 46) & (300, 25) \\ 
Random 3 & (3, 3) & (300, 46) & (300, 25) \\ 
Random 4 & (3, 3) & (300, 47) & (300, 4) \\ 
Random 5 & (3, 3) & (300, 47) & (300, 25) \\ 
Random 6 & (3, 3) & (300, 45) & (300, 23) \\ 
Random 7 & (3, 3) & (300, 45) & (300, 25) \\ 
Random 8 & (3, 3) & (300, 45) & (300, 21) \\ 
Random 9 & (3, 3) & (300, 45) & (300, 26) \\ 
Random 10 & (3, 3) & (300, 47) & (300, 25) \\ 
	\hline
\end{tabular}
\end{tabular}

\begin{tabular}{ll}
\tiny
\setlength{\tabcolsep}{3.0pt}

\begin{tabular}{cccccccc|}
	\hline
Data & Layer 1 & Layer 2 & Layer 3 & Layer 4 & Layer 5 & Layer 6 \\ 
	\hline
spiral 1 & (2, 2) & (300, 15) & (300, 6) & (300, 7) & (300, 6) \\ 
spiral 2 & (2, 2) & (300, 13) & (300, 6) & (300, 7) & (300, 6) & (300, 6) \\ 
spiral 3 & (2, 2) & (300, 12) & (300, 6) & (300, 7) & (300, 6) & (300, 6) \\ 
spiral 4 & (2, 2) & (300, 13) & (300, 6) & (300, 7) & (300, 6) & (300, 6) \\ 
spiral 5 & (2, 2) & (300, 13) & (300, 6) & (300, 7) & (300, 6) \\ 
spiral 6 & (2, 2) & (300, 14) & (300, 6) & (300, 7) & (300, 6) \\ 
spiral 7 & (2, 2) & (300, 14) & (300, 6) & (300, 7) & (300, 6) \\ 
spiral 8 & (2, 2) & (300, 14) & (300, 6) & (300, 7) & (300, 6) & (300, 6) \\ 
spiral 9 & (2, 2) & (300, 13) & (300, 6) & (300, 7) & (300, 6) \\ 
spiral 10 & (2, 2) & (300, 14) & (300, 6) & (300, 7) & (300, 6) \\ 
	\hline
\end{tabular}
&
\tiny
\setlength{\tabcolsep}{3.0pt}

\begin{tabular}{cccccccc}
	\hline
Data & Layer 1 & Layer 2 & Layer 3 & Layer 4 & Layer 5 & Layer 6 \\ 
	\hline
wine 1 & (13, 11) & (300, 76) & (300, 6) & (300, 7) & (300, 6) & (300, 6) \\ 
wine 2 & (13, 11) & (300, 76) & (300, 6) & (300, 6) & (300, 6) & (300, 6) \\ 
wine 3 & (13, 11) & (300, 75) & (300, 6) & (300, 7) & (300, 6) & (300, 6) \\ 
wine 4 & (13, 11) & (300, 76) & (300, 6) & (300, 6) & (300, 6) & (300, 6) \\ 
wine 5 & (13, 11) & (300, 74) & (300, 6) & (300, 7) & (300, 6) & (300, 6) \\ 
wine 6 & (13, 11) & (300, 74) & (300, 6) & (300, 6) & (300, 6) & (300, 6) \\ 
wine 7 & (13, 11) & (300, 74) & (300, 6) & (300, 6) & (300, 6) & (300, 6) \\ 
wine 8 & (13, 11) & (300, 75) & (300, 6) & (300, 7) & (300, 6) & (300, 6) \\ 
wine 9 & (13, 11) & (300, 75) & (300, 6) & (300, 8) & (300, 6) & (300, 6) \\ 
wine 10 & (13, 11) & (300, 76) & (300, 6) & (300, 7) & (300, 6) & (300, 6) \\ 
	\hline
\end{tabular}
\end{tabular}

\begin{tabular}{ll}
\tiny
\setlength{\tabcolsep}{3.0pt}

\begin{tabular}{cccccccc|}
	\hline
Data & Layer 1 & Layer 2 & Layer 3 & Layer 4 & Layer 5 & Layer 6 \\ 
	\hline
car 1 & (6, 6) & (300, 96) & (300, 6) & (300, 8) & (300, 6) \\ 
car 2 & (6, 6) & (300, 96) & (300, 6) & (300, 8) & (300, 6) \\ 
car 3 & (6, 6) & (300, 91) & (300, 6) & (300, 8) & (300, 6) \\ 
car 4 & (6, 6) & (300, 88) & (300, 6) & (300, 8) & (300, 6) & (300, 6) \\ 
car 5 & (6, 6) & (300, 94) & (300, 6) & (300, 8) & (300, 6) \\ 
car 6 & (6, 6) & (300, 93) & (300, 6) & (300, 7) \\ 
car 7 & (6, 6) & (300, 92) & (300, 6) & (300, 8) & (300, 6) \\ 
car 8 & (6, 6) & (300, 95) & (300, 6) & (300, 7) & (300, 6) \\ 
car 9 & (6, 6) & (300, 96) & (300, 6) & (300, 9) & (300, 6) \\ 
car 10 & (6, 6) & (300, 99) & (300, 6) & (300, 8) & (300, 6) \\ 
	\hline
\end{tabular}
&
\tiny
\setlength{\tabcolsep}{3.0pt}

\begin{tabular}{ccccccc|}
	\hline
Data & Layer 1 & Layer 2 & Layer 3 & Layer 4 & Layer 5 \\ 
	\hline
divorce 1 & (54, 35) & (300, 44) & (300, 5) & (300, 5) \\ 
divorce 2 & (54, 35) & (300, 45) & (300, 4) & (300, 4) \\ 
divorce 3 & (54, 36) & (300, 49) & (300, 6) & (300, 6) \\ 
divorce 4 & (54, 36) & (300, 47) & (300, 7) & (300, 6) \\ 
divorce 5 & (54, 35) & (300, 45) & (300, 6) & (300, 6) \\ 
divorce 6 & (54, 36) & (300, 47) & (300, 6) & (300, 6) \\ 
divorce 7 & (54, 35) & (300, 45) & (300, 6) & (300, 6) & (300, 4) \\ 
divorce 8 & (54, 36) & (300, 47) & (300, 6) & (300, 7) & (300, 4) \\ 
divorce 9 & (54, 36) & (300, 47) & (300, 5) & (300, 5) \\ 
divorce 10 & (54, 36) & (300, 47) & (300, 6) & (300, 6) \\ 
	\hline
\end{tabular}
\end{tabular}

\begin{table}[h]
\tiny
\setlength{\tabcolsep}{3.0pt}

\begin{tabular}{cccccccccccc|}
	\hline
Data & Layer 1 & Layer 2 & Layer 3 & Layer 4 & Layer 5 & Layer 6 & Layer 7 & Layer 8 & Layer 9 & Layer 10 \\ 
	\hline
cancer 1 & (9, 8) & (300, 90) & (300, 5) & (300, 6) & (300, 6) & (300, 5) & (300, 4) & (300, 5) & (300, 6) & (300, 6) \\ 
cancer 2 & (9, 8) & (300, 90) & (300, 6) & (300, 7) & (300, 8) & (300, 11) & (300, 8) & (300, 4) \\ 
cancer 3 & (9, 8) & (300, 88) & (300, 5) & (300, 6) & (300, 7) & (300, 7) & (300, 6) & (300, 4) \\ 
cancer 4 & (9, 8) & (300, 93) & (300, 6) & (300, 7) & (300, 9) & (300, 11) & (300, 8) \\ 
cancer 5 & (9, 8) & (300, 93) & (300, 9) & (300, 10) & (300, 10) & (300, 11) & (300, 9) & (300, 7) \\ 
cancer 6 & (9, 8) & (300, 92) & (300, 7) & (300, 8) & (300, 8) & (300, 7) & (300, 7) \\ 
cancer 7 & (9, 8) & (300, 90) & (300, 4) & (300, 4) & (300, 5) & (300, 6) & (300, 6) & (300, 6) & (300, 6) \\ 
cancer 8 & (9, 8) & (300, 88) & (300, 5) & (300, 6) & (300, 7) & (300, 8) & (300, 7) & (300, 6) \\ 
cancer 9 & (9, 8) & (300, 88) & (300, 5) & (300, 7) & (300, 7) & (300, 7) & (300, 7) \\ 
cancer 10 & (9, 8) & (300, 97) & (300, 9) & (300, 11) & (300, 12) & (300, 13) & (300, 6) \\ 
	\hline
\end{tabular}
\end{table}

\begin{table}[h]
\tiny
\setlength{\tabcolsep}{3.0pt}

\begin{tabular}{cccccc|}
	\hline
Data & Layer 1 & Layer 2 & Layer 3 & Layer 4 \\ 
	\hline
face 1 & (960, 233) & (300, 74) & (300, 73) & (300, 46) \\ 
face 2 & (960, 231) & (300, 75) & (300, 73) & (300, 43) \\ 
face 3 & (960, 231) & (300, 76) & (300, 73) & (300, 44) \\ 
face 4 & (960, 232) & (300, 76) & (300, 74) & (300, 44) \\ 
face 5 & (960, 231) & (300, 77) & (300, 73) & (300, 43) \\ 
face 6 & (960, 232) & (300, 74) & (300, 72) & (300, 47) \\ 
face 7 & (960, 232) & (300, 76) & (300, 73) & (300, 45) \\ 
face 8 & (960, 230) & (300, 74) & (300, 74) & (300, 44) \\ 
face 9 & (960, 233) & (300, 76) & (300, 76) & (300, 45) \\ 
face 10 & (960, 231) & (300, 76) & (300, 70) & (300, 43) \\ 
	\hline
\end{tabular}
\end{table}

\end{appendices}

\clearpage
\newpage
