# Supplementary material for: Kernel Dependence Network
Source: arXiv:2011.03320 source file (2020-11-09)
Supplement: Supplementary file 14 [file l_kernel_graphs.tex]

\clearpage
%\newpage

\begin{appendices}
\section{Graphs of Kernel Sequences}
\label{app:kernel_sequence_graph}

A representation of the \KS are displayed in the figures below for each dataset. The samples of the kernel matrix are previously organized to form a block structure by placing samples of the same class adjacent to each other. Since the Gaussian kernel is restricted to values between 0 and 1, we let white and dark blue be 0 and 1 respectively where the gradients reflect values in between. Our theorems predict that the \KS will evolve from an uninformative kernel into a highly discriminating kernel of perfect block structures. 

\begin{figure}[h]
\center
    \includegraphics[width=9cm]{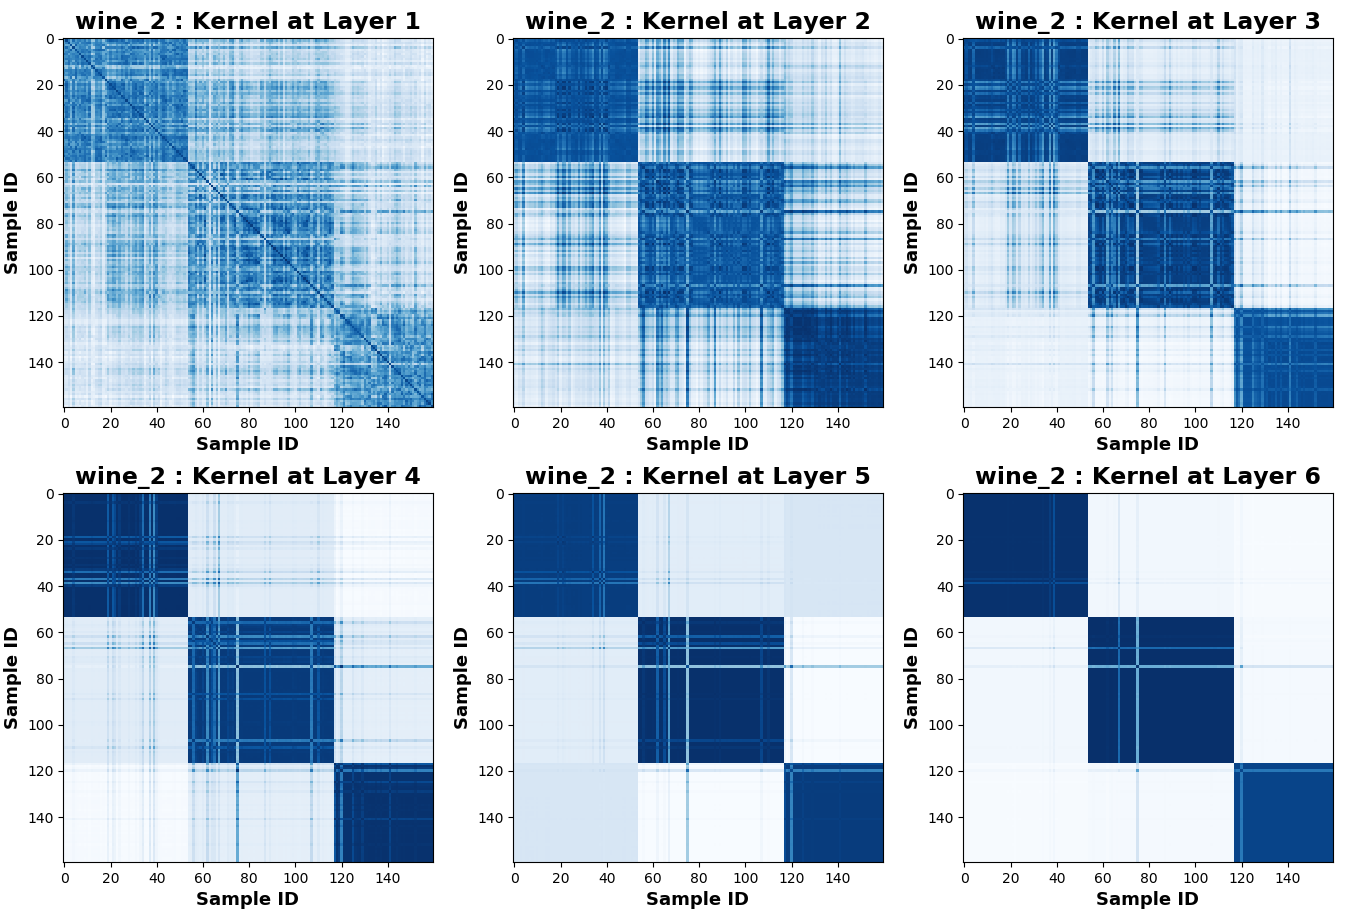}
    \caption{The kernel sequence for the wine dataset.}
\end{figure} 

\begin{figure}[h]
\center
    \includegraphics[width=9cm]{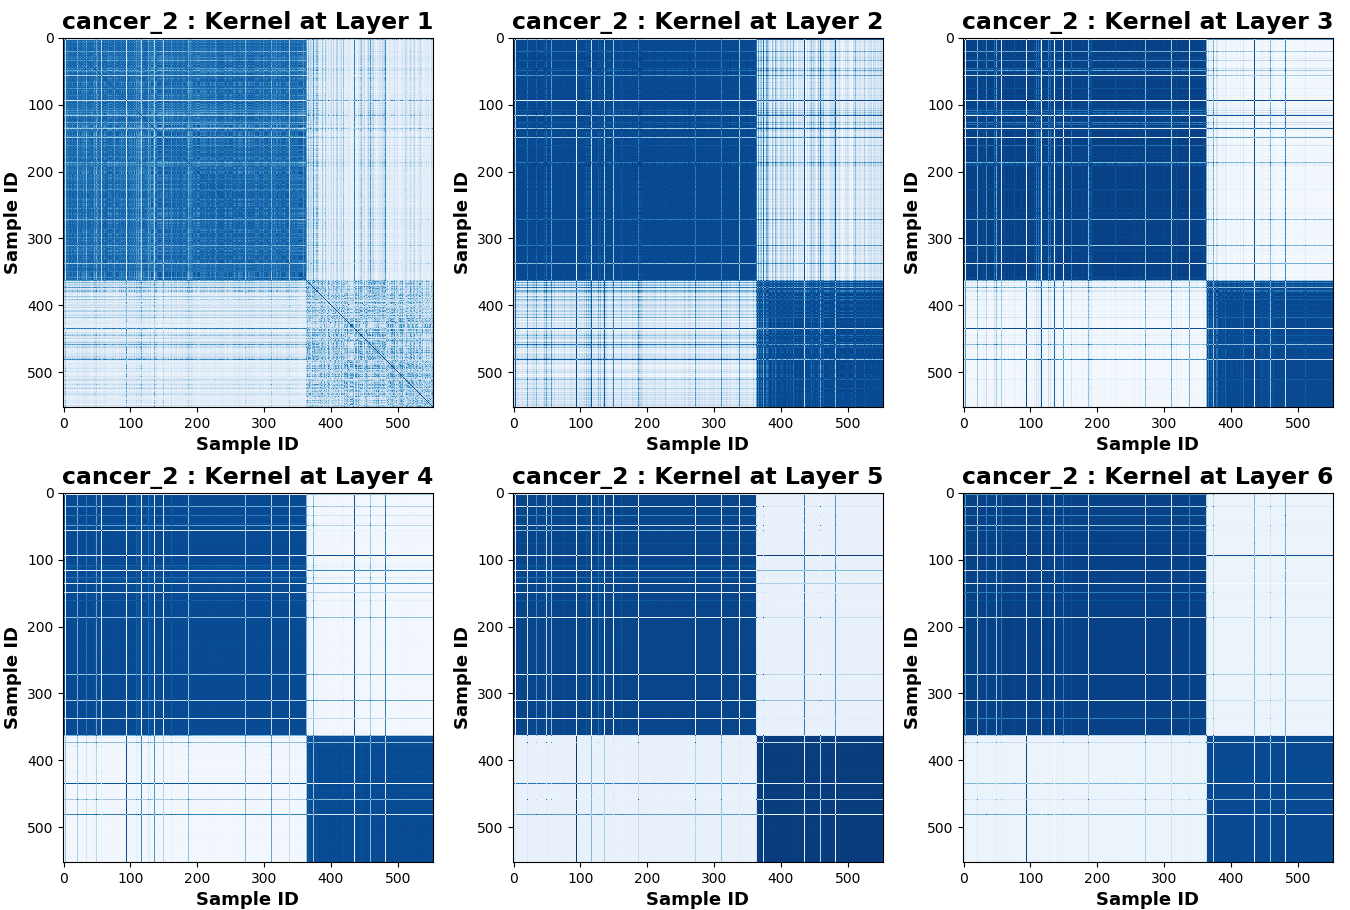}
    \caption{The kernel sequence for the cancer dataset.}
\end{figure} 

\begin{figure}[h]
\center
    \includegraphics[width=9cm]{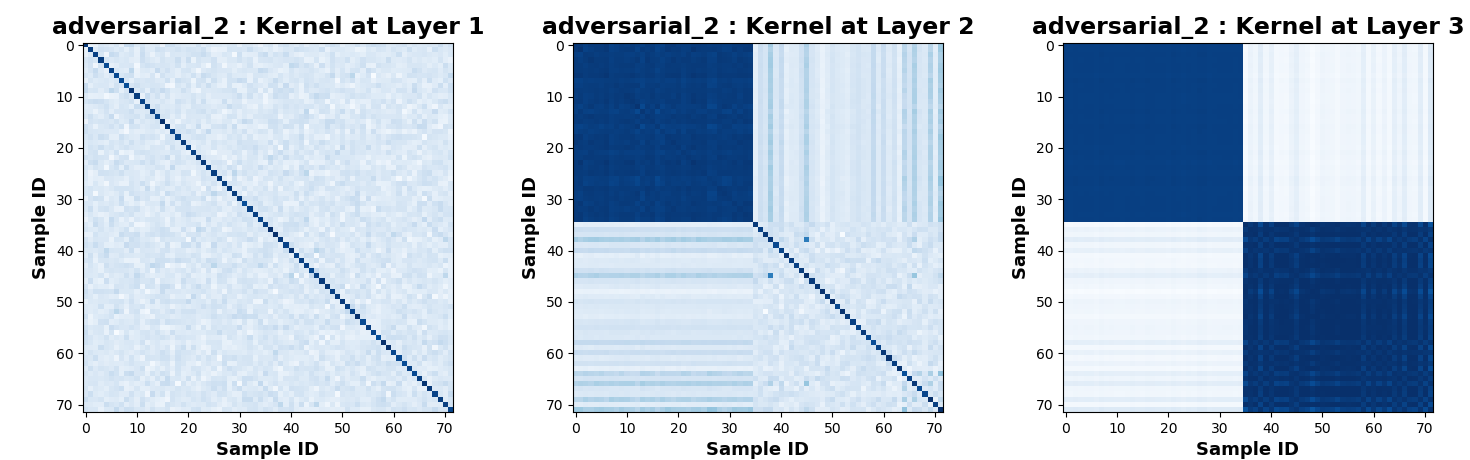}
    \caption{The kernel sequence for the Adversarial dataset.}
\end{figure} 

\begin{figure}[h]
\center
    \includegraphics[width=9cm]{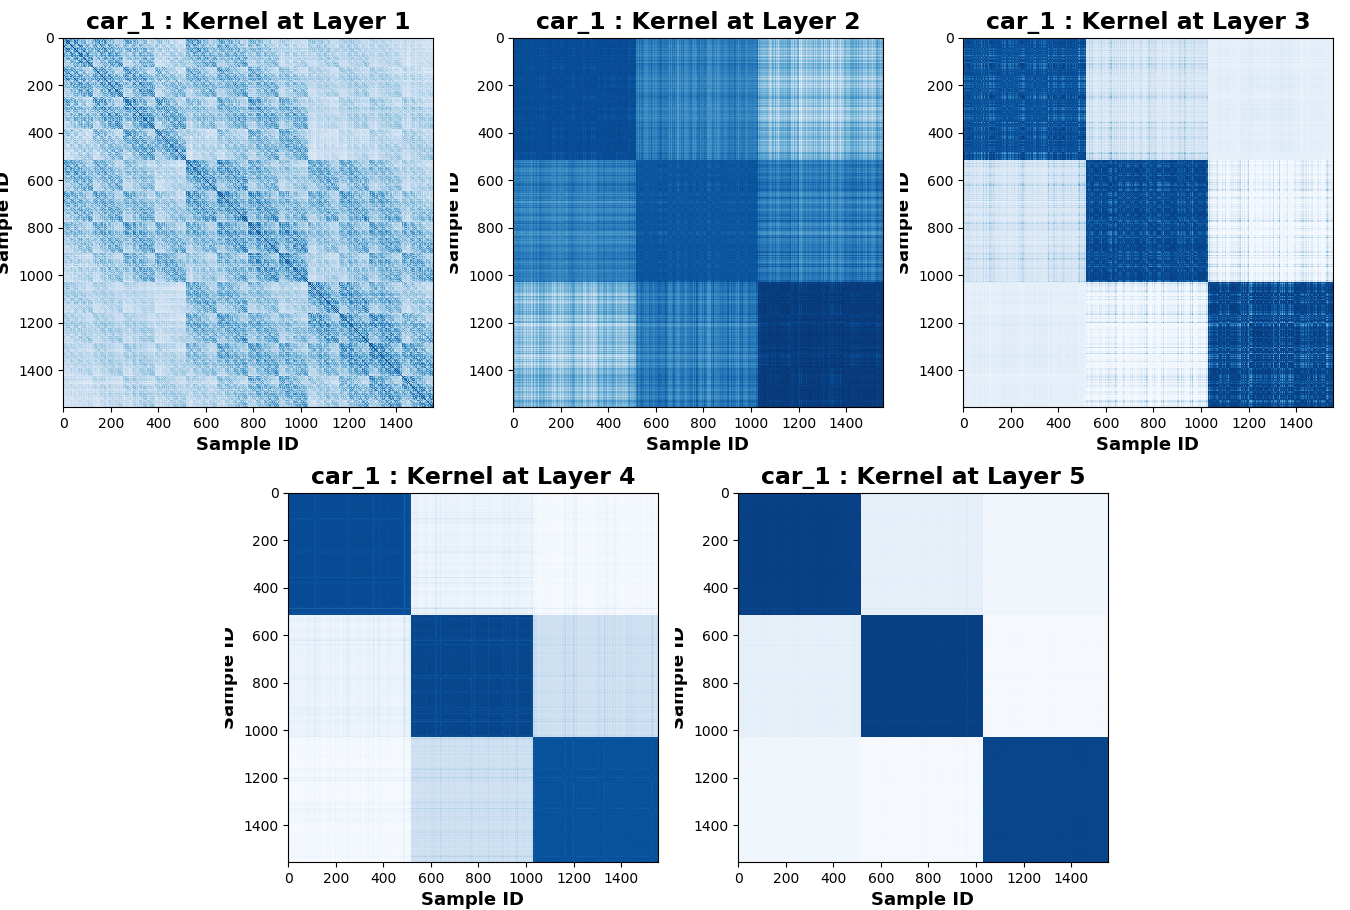}
    \caption{The kernel sequence for the car dataset.}
\end{figure} 

\begin{figure}[h]
\center
    \includegraphics[width=11cm]{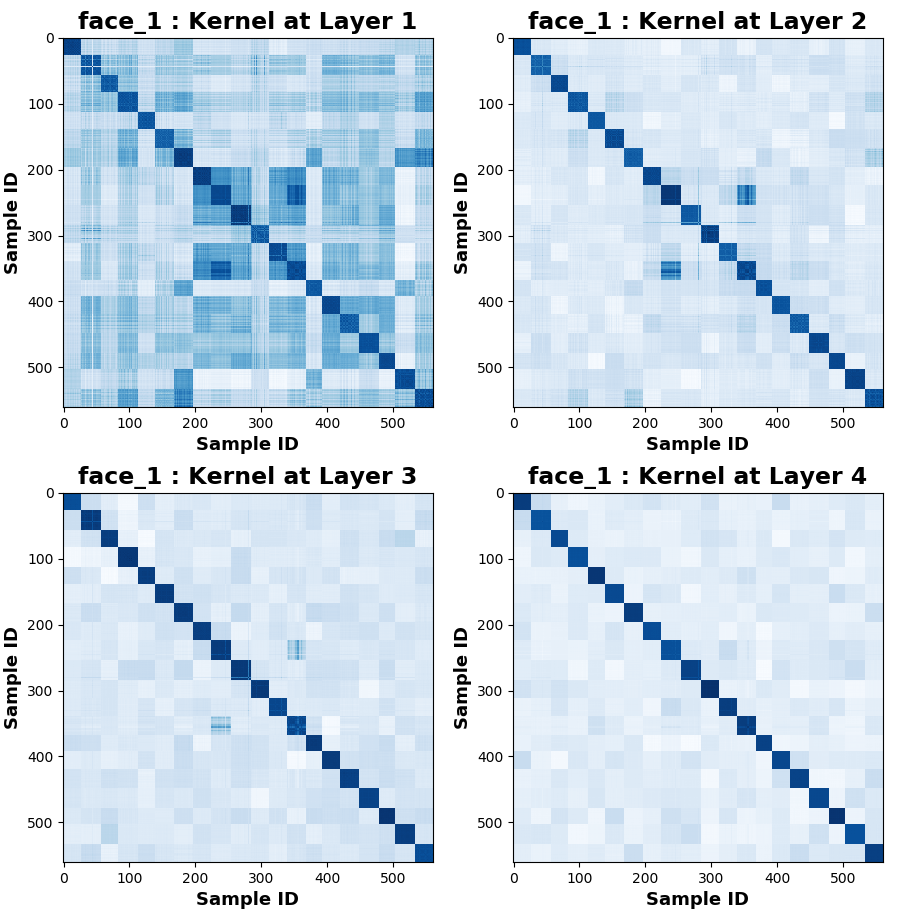}
    \caption{The kernel sequence for the face dataset.}
\end{figure} 

\begin{figure}[h]
\center
    \includegraphics[width=9cm]{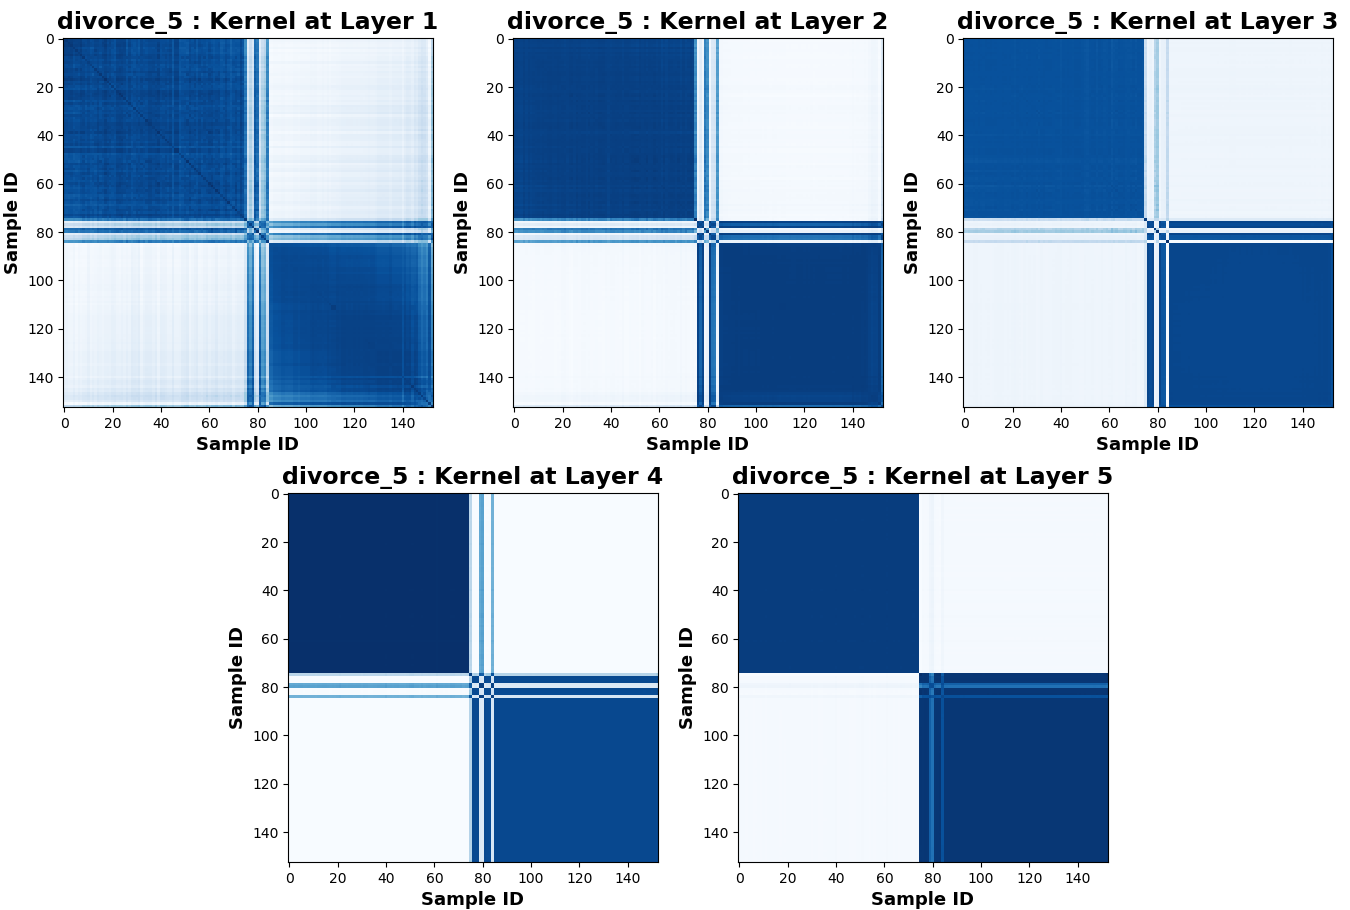}
    \caption{The kernel sequence for the divorce dataset.}
\end{figure} 

\begin{figure}[h]
\center
    \includegraphics[width=11cm]{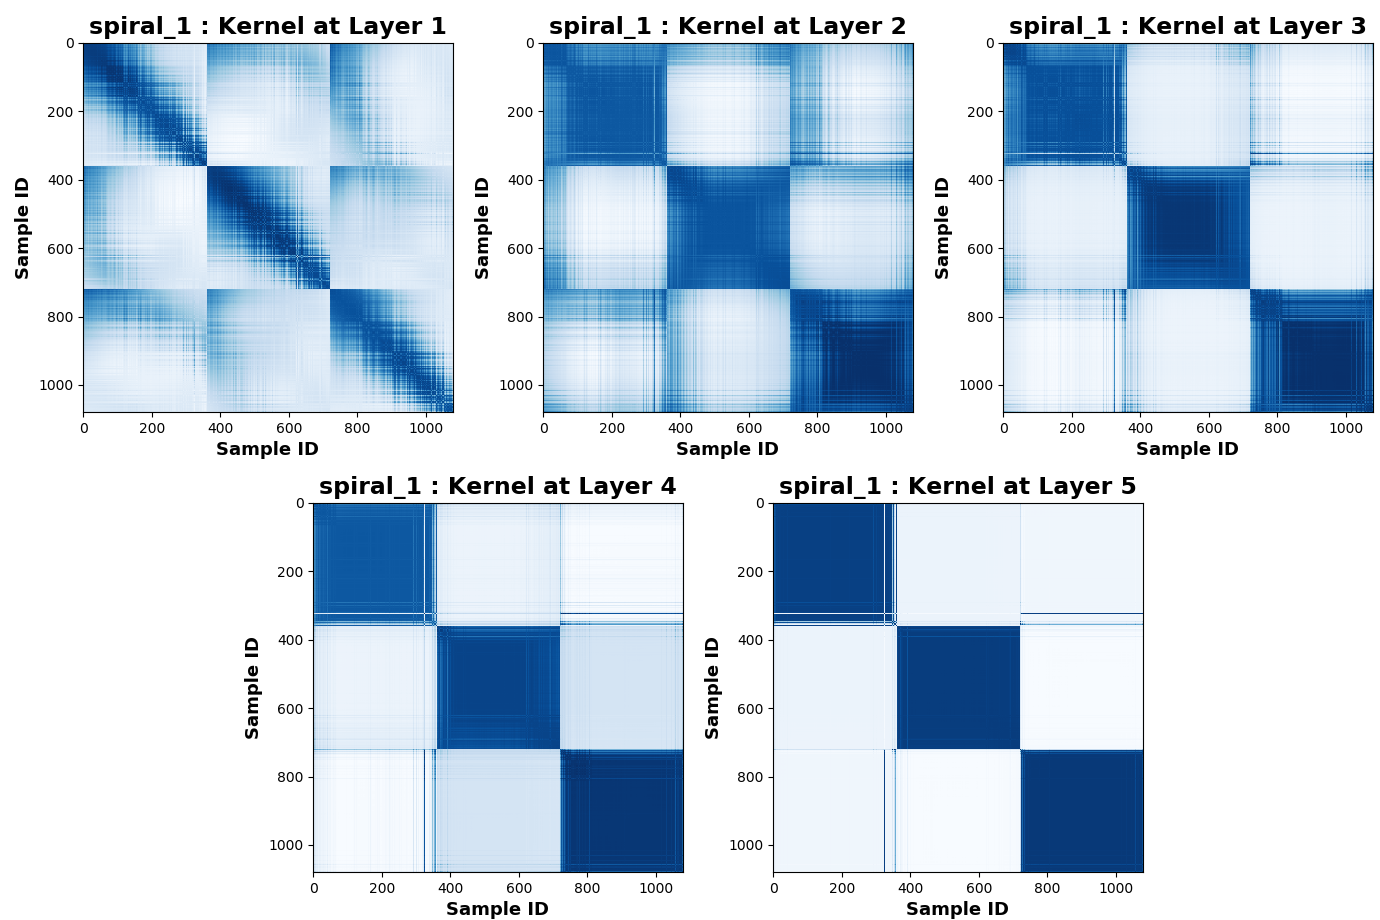}
    \caption{The kernel sequence for the spiral dataset.}
\end{figure}

\begin{figure}[h]
\center
    \includegraphics[width=11cm]{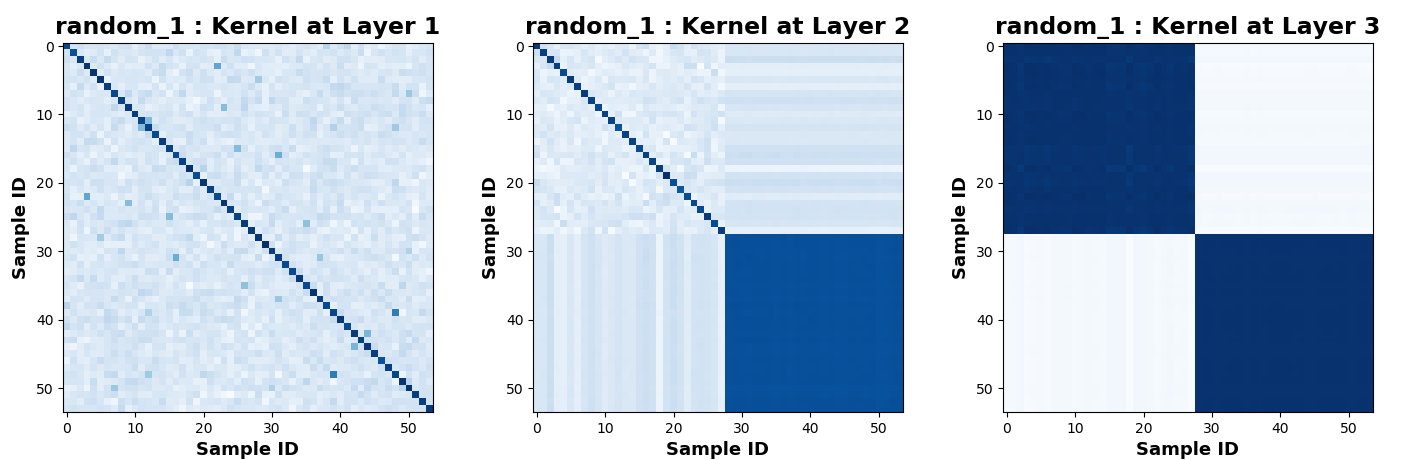}
    \caption{The kernel sequence for the Random dataset.}
\end{figure} 
\end{appendices}
