# Supplementary material for: Kernel Dependence Network
Source: arXiv:2011.03320 source file (2020-11-09)
Supplement: Supplementary file 15 [file n_optimal_sigma.tex]

\newpage
\begin{appendices}
\section{Optimal Gaussian $\sigma$ for Maximum Kernel Separation}
\label{app:opt_sigma}
Although the Gaussian kernel is the most common kernel choice for kernel methods, its $\sigma$ value is a hyperparameter that must be tuned for each dataset. This work proposes to set the $\sigma$ value based on the maximum kernel separation. The source code is made publicly available on \url{https://github.com/anonamous}.
%\url{https://github.com/endsley/opt_gaussian_-}.

Let $X \in \mathbb{R}^{n \times d}$ be a dataset of $n$ samples with $d$ features and let $Y \in \mathbb{R}^{n \times \nclass}$ be the corresponding one-hot encoded labels where $\nclass$ denotes the number of classes. Given $\kappa_X(\cdot, \cdot)$ and $\kappa_Y(\cdot,\cdot)$ as two kernel functions that applies respectively to $X$ and $Y$ to construct kernel matrices $K_X \in \mathbb{R}^{n \times n}$ and $K_Y \in \mathbb{R}^{n \times n}$. Given a set $\mathcal{S}$, we denote $|\mathcal{S}|$ as the number of elements within the set. Also let $\mathcal{S}$ and $\mathcal{S}^c$ be sets of all pairs of samples of $(x_i,x_j)$ from a dataset $X$ that belongs to the same and different classes respectively, then the average kernel value for all $(x_i,x_j)$ pairs with the same class is
\begin{equation}
    d_{\mathcal{S}} = \frac{1}{|\mathcal{S}|}\sum_{i,j \in \mathcal{S}} e^{-\frac{||x_i - x_j||^2}{2\sigma^2}}
\end{equation}
and the average kernel value for all $(x_i,x_j)$ pairs between different classes is
\begin{equation}
    d_{\mathcal{S}^c} = 
    \frac{1}{|\mathcal{S}^c|}\sum_{i,j \in \mathcal{S}^c} e^{-\frac{||x_i - x_j||^2}{2\sigma^2}}. 
\end{equation}
We propose to find the $\sigma$ that maximizes the difference between $d_{\mathcal{S}}$ and $d_{\mathcal{S}^c}$ or 
\begin{equation}
    \underset{\sigma}{\max} \quad 
    \frac{1}{|\mathcal{S}|}\sum_{i,j \in \mathcal{S}} e^{-\frac{||x_i - x_j||^2}{2\sigma^2}} - 
    \frac{1}{|\mathcal{S}^c|}\sum_{i,j \in \mathcal{S}^c} e^{-\frac{||x_i - x_j||^2}{2\sigma^2}}.
    \label{eq:main_objective}
\end{equation}
It turns out that is expression can be computed efficiently. Let $g = \frac{1}{|\mathcal{S}|}$ and $\bar{g} = \frac{1}{|\mathcal{S}^c|}$, and let $\textbf{1}_{n \times n} \in \mathbb{R}^{n \times n}$ be a matrix of 1s, then we can define $Q$ as
\begin{equation}
    Q = -g K_Y + \bar{g} (\textbf{1}_{n \times n} - K_Y).
\end{equation}
Or $Q$ can be written more compactly as
\begin{equation}
    Q = \bar{g} \textbf{1}_{n \times n} - (g + \bar{g})K_Y. 
\end{equation}
Given $Q$, Eq.~(\ref{eq:main_objective}) becomes
\begin{equation}
    \underset{\sigma}{\min} \quad 
    \Tr(K_X Q).
    \label{eq:obj_compact}
\end{equation}
This objective can be efficiently solved with BFGS. 

Below in Fig.~\ref{fig:max_kernel_separation}, we plot out the average within cluster kernel and the between cluster kernel values as we vary $\sigma$. From the plot, we can see that the maximum separation is discovered via BFGS. 
    \begin{figure}[h]
        \centering
        \includegraphics[width=10cm,height=7cm]{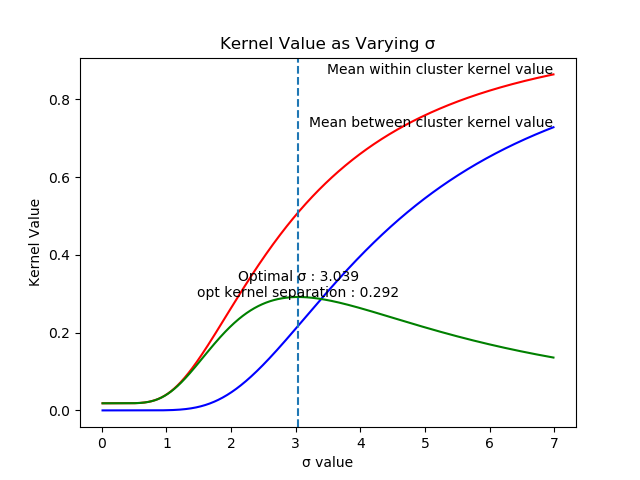}
        \caption{Maximum Kernel separation.}
        \label{fig:max_kernel_separation}
    \end{figure}

\textbf{Relation to HSIC. }    
From Eq.~(\ref{eq:obj_compact}), we can see that the $\sigma$ that causes maximum kernel separation is directly related to HSIC. Given that the HSIC objective is normally written as
\begin{equation}
    \underset{\sigma}{\min} \quad 
    \Tr(K_X H K_Y H),
\end{equation}
by setting $Q=HK_YH$, we can see how the two formulations are related. While the maximum kernel separation places the weight of each sample pair equally, HSIC weights the pair differently.
We also notice that the $Q_{i,j}$ element is positive/negative for $(x_i,x_j)$ pairs that are with/between classes respectively. Therefore, the argument for the global optimum should be relatively close for both objectives. Below in Figure~\ref{fig:max_HSIC}, we show a figure of HSIC values as we vary $\sigma$. Notice how the optimal $\sigma$ is almost equivalent to the solution from maximum kernel separation. For the purpose of \kc, we use $\sigma$ that maximizes the HSIC value.
    \begin{figure}[h]
        \centering
        \includegraphics[width=10cm,height=7cm]{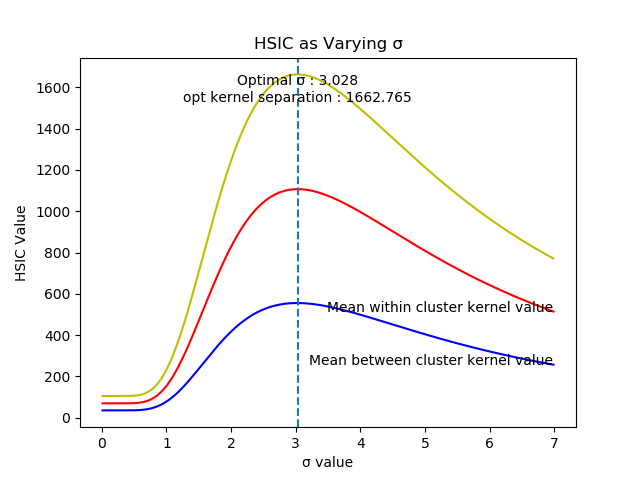}
        \caption{Maximal HSIC.}
        \label{fig:max_HSIC}
    \end{figure} 
\end{appendices}
