# Supplementary material for: Kernel Dependence Network
Source: arXiv:2011.03320 source file (2020-11-09)
Supplement: Supplementary file 16 [file 2nd_necessary.tex]

\begin{appendices}
\section{2nd Order Necessary Conditions}\label{app:2nd_order}
\begin{lemma} 
  [Bertsekas, Proposition 3.1.1~{\cite{bertsekas1997nonlinear}}] (Lagrange Multiplier Theorem - Necessary Conditions)
    Consider the optimization problem:
  $ \min_{W : h (W) = 0} f (W), $
where $f : \mathbb{R}^{d \times q} \to \mathbb{R}$ and $h :
  \mathcal{R}^{d \times q} \to \mathbb{R}^{q \times q}$ are twice continuously
  differentiable. Let   $\mathcal{L}$ be the Lagrangian and $h(W)$ its equality constraint. Then, a local minimum must satisfy the following  conditions:
  \begin{subequations}
    \begin{align} 
    &\nabla_W \mathcal{L} (W^{\ast}, \Lambda^{\ast}) = 0, \label{eq:1st_W}\\
    &\nabla_{\Lambda} \mathcal{L} (W^{\ast}, \Lambda^{\ast}) = 0, \label{eq:1st_lambda}\\
    \begin{split}
     \tmop{Tr}( Z^T &\nabla_{W W}^2 \mathcal{L}(W^{\ast}, \Lambda^{\ast}) Z) \geq 0 \\ 
     &\tmop{for}   \tmop{all} Z \neq 0 , \tmop{with}  \nabla h (W^{\ast})^T Z = 0.   \label{eq:2nd_W_in_append} 
    \end{split}
    \end{align}   
  \end{subequations}
\end{lemma}
\end{appendices}
