# Supplementary material for: Kernel Dependence Network
Source: arXiv:2011.03320 source file (2020-11-09)
Supplement: Supplementary file 17 [file d_app_4.tex]

%\begin{appendices}
%\section{Proof for Property \ref{prop:kernel_in_RKHS} and \ref{prop:kernel_in_IDS}}
%\label{app:kernel_define_metric_in_IDS}
%\begin{proof}
%From Appendix~\ref{app:ccn_satisfies_dependence_property}, we concluded that HSIC can be rewritten into the equation that satisfies the \textit{separability property} where we optimize   
%     \begin{equation}
%        \underset{W}{\max} \quad \sum_{i,j \in \mathcal{S}} \Gamma_{i,j} 
%        \langle \Psi(W^Tx_i), \Psi(W^Tx_j) \rangle - 
%        \sum_{i,j \in \bar{\mathcal{S}}}
%        \Gamma_{i,j} 
%        \langle \Psi(W^Tx_i), \Psi(W^Tx_j) \rangle
%        \hspace{0.2cm} \text{s.t} \hspace{0.2cm} W^TW = I.
%        \label{eq:inner_controls_the_metric}
%    \end{equation}   
%From Eq.~(\ref{eq:inner_controls_the_metric}), we see that the inner product is always used as the metric in RKHS. However, if the kernel is written as a function, it is also equivalent to 
%     \begin{equation}
%        \underset{W}{\max} \quad \sum_{i,j \in \mathcal{S}} \Gamma_{i,j} 
%        \kappa(W^Tx_i, W^Tx_j)  - 
%        \sum_{i,j \in \bar{\mathcal{S}}}
%        \Gamma_{i,j} 
%        \kappa(W^Tx_i, W^Tx_j)
%        \hspace{0.2cm} \text{s.t} \hspace{0.2cm} W^TW = I.
%        \label{eq:inner_controls_the_IDS}
%    \end{equation}   
%Since Eq.~(\ref{eq:inner_controls_the_IDS}) reflects the result in IDS, the kernel function directly controls how the distance between samples are measured. Given this control, it defines the metric which satisfies the \textit{separability property}.
%\end{proof}
%\end{appendices}
