# Supplementary material for: Kernel Dependence Network
Source: arXiv:2011.03320 source file (2020-11-09)
Supplement: Supplementary file 18 [file h_app_8.tex]

%\begin{appendices}
%\section{Details on SPCA and Kernelized SPCA}
%\label{app:SPCA_SKPCA}
%Supervised PCA is also based on an HSIC formulation where we perform dimension reduction within RKHS with
%\begin{equation}
%    \underset{W}{\max} \quad \Tr( \Psi W W^T \Psi^T H K_Y H)
%    \hspace{1cm} \text{s.t} \hspace{1cm} W^TW = I, 
%     \label{eq:hsic_trace_with_SPCA}
%\end{equation}
%where $\Psi$ is the image of the data mapped into RKHS. With this formulation, we seek to find the low dimension subspace that is maximally dependent on the labels Y. By applying the rotation property of the Trace operator, this equation can be reformulated into
%\begin{equation}
%    \underset{W}{\max} \quad \Tr( W^T \Psi^T H K_Y H \Psi W)
%    \hspace{1cm} \text{s.t} \hspace{1cm} W^TW = I. 
%\end{equation}
%Since $\Psi$ may potentially have infinite dimensions dependent on the kernel choice, the original Supervised PCA used a linear kernel where $\Psi = X$. Therefore, given the application of Random Fourier Feature to approximate potentially infinite dimensions, $\Psi$ becomes a finite dimension matrix; thereby enabling the feasibility of its computation. To solve this problem, the solution is simply the most dominant eigenvectors of the matrix $\Psi^THK_YH\Psi$.
%\end{appendices}
