# Supplementary material for: Kernel Dependence Network
Source: arXiv:2011.03320 source file (2020-11-09)
Supplement: Supplementary file 19 [file m_metric_graphs.tex]

\clearpage
\newpage

\begin{appendices}
\section{Evaluation Metrics Graphs}
\label{app:metric_graphs}

\begin{figure}[h]
\center
    \includegraphics[width=10cm]{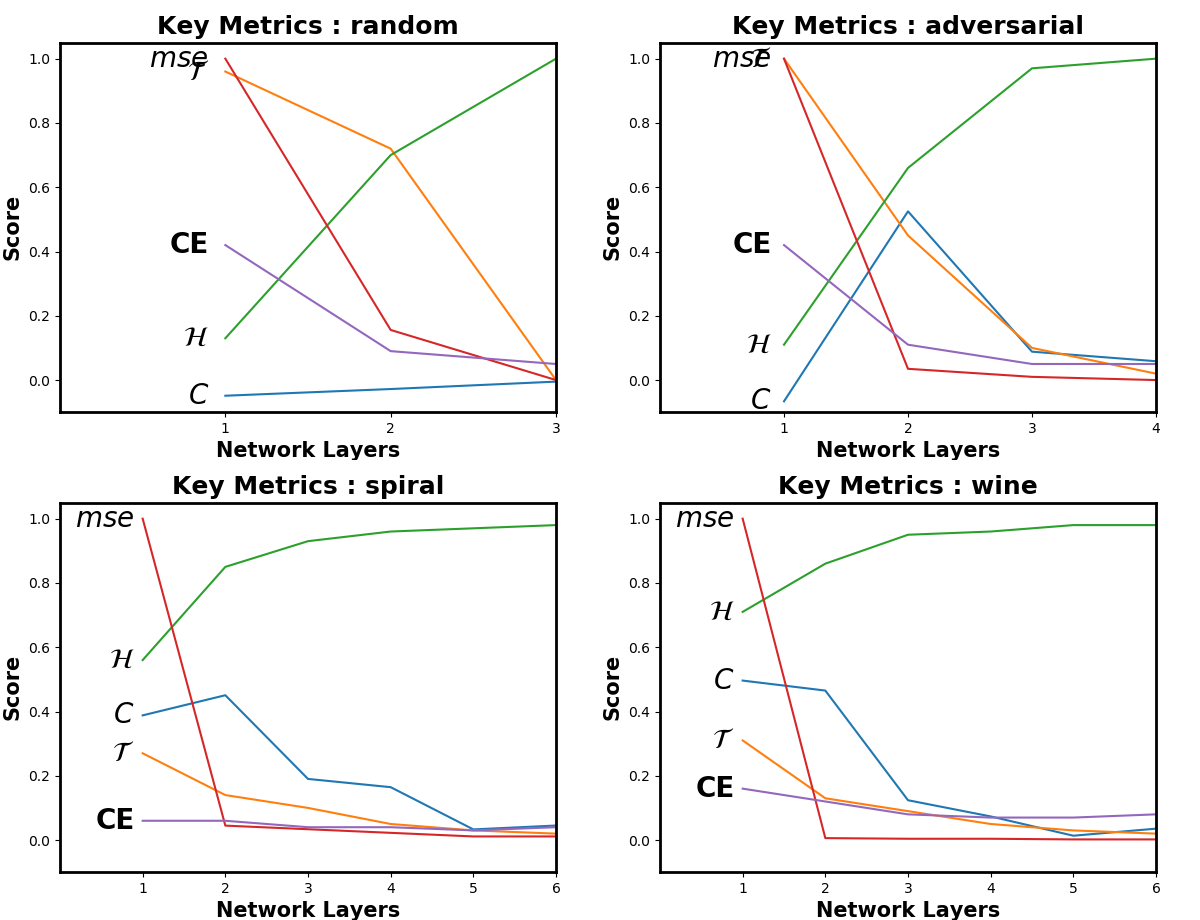}
    \caption{}
\end{figure} 

\begin{figure}[h]
\center
    \includegraphics[width=10cm]{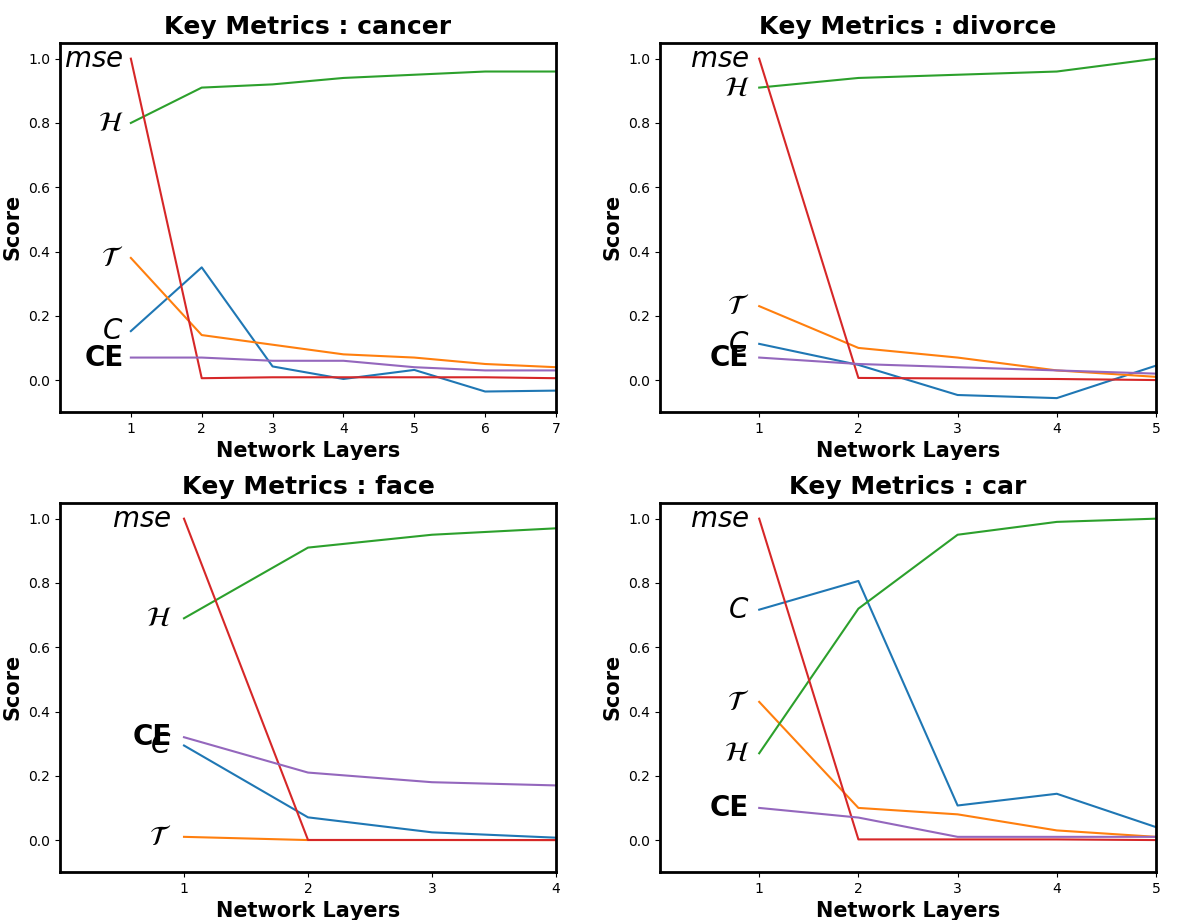}
    \caption{Figures of key metrics for all datasets as samples progress through the network. It is important to notice the uniformly and monotonically increasing \RS for each plot
    since this guarantees a converging kernel/risk sequence. As the $\mathcal{T}$ approach 0, samples of the same/difference classes in IDS are being pulled into a single point or pushed maximally apart respectively. As $C$ approach 0, samples of the same/difference classes in RKHS are being pulled into 0 or $\frac{\pi}{2}$ cosine similarity respectively.}
\end{figure} 

\end{appendices}
